# Supplementary material for: Development and validation of a high-fidelity full-spectrum Monte Carlo model for the Swiss airborne gamma-ray spectrometry system
Source: arXiv:2502.02102 ancillary file (2025-06-22)
Supplement: Supplementary file 1 [file Supplementary_Information.pdf]

# Supplementary Information for

## Development and validation of a high-fidelity full-spectrum Monte Carlo model for the Swiss airborne gamma-ray spectrometry system

David Breitenmoser<sup>1,2,\*</sup>, Alberto Stabilini<sup>1</sup>, Malgorzata Magdalena Kasprzak<sup>1</sup>, Sabine Mayer<sup>1</sup>

<sup>1</sup>Department of Radiation Safety and Security, Paul Scherrer Institute (PSI), Forschungsstrasse 111, Villigen PSI, 5232, Switzerland

<sup>2</sup>Department of Physics, Swiss Federal Institute of Technology (ETH), Otto-Stern-Weg 5, Zurich, 8093, Switzerland

\*Corresponding author: David Breitenmoser (E-Mail: david.breitenmoser@psi.ch, ORCID: 0000-0003-0339-6592)

### The PDF includes:

- Supplementary Methods S1.1–S1.4
- Supplementary Figures S1–S8
- Supplementary Tables S1–S6
- Supplementary References

# Contents

|                                                  |      |
|--------------------------------------------------|------|
| List of Supplementary Figures                    | SIII |
| List of Supplementary Tables                     | SIV  |
| S1 Supplementary Methods                         | S1   |
| S1.1 Postprocessing Pipeline: RLLSpec . . . . .  | S1   |
| S1.2 Calibration Pipeline: RLLCal . . . . .      | S3   |
| S1.2.1 Spectral Energy Calibration . . . . .     | S3   |
| S1.2.2 Spectral Resolution Calibration . . . . . | S6   |
| S1.2.3 LLD Calibration . . . . .                 | S8   |
| S1.3 Postprocessing Pipeline: NPScinMC . . . . . | S11  |
| S1.4 Uncertainty Quantification . . . . .        | S16  |
| S1.4.1 Measurement Uncertainty . . . . .         | S16  |
| S1.4.2 Simulation Uncertainty . . . . .          | S20  |
| S2 Supplementary Figures                         | S24  |
| S3 Supplementary Tables                          | S29  |
| Supplementary References                         | S32  |

## List of Supplementary Figures

|    |                                                                           |     |
|----|---------------------------------------------------------------------------|-----|
| S1 | Energy calibration models . . . . .                                       | S5  |
| S2 | Spectral resolution models . . . . .                                      | S7  |
| S3 | $\chi^2$ -contour maps of the LLD model parameters . . . . .              | S10 |
| S4 | System architecture of the Swiss AGRS system . . . . .                    | S24 |
| S5 | Fuel level model of the AS332M1 aircraft . . . . .                        | S25 |
| S6 | Technical drawing of the custom-built $K_{\text{nat}}$ sources . . . . .  | S26 |
| S7 | Environment mass model sensitivity analysis . . . . .                     | S27 |
| S8 | Refined pulse-height channel number bin width convergence study . . . . . | S28 |

List of Supplementary Tables

S1 K<sub>nat</sub> radionuclide source specification . . . . . S29

S2 Near-field radiation measurements . . . . . S29

S3 Mid-field radiation measurements . . . . . S30

S4 Far-field radiation measurements . . . . . S30

S5 Calibration sources . . . . . S31

S6 Calibration results derived by the RLLCa1 pipeline . . . . . S31

# S1 Supplementary Methods

## S1.1 Postprocessing Pipeline: RLLSpec

To postprocess the pulse-height spectra measured by the gamma-ray spectrometer, a dedicated pipeline named RLLSpec was developed using the MATLAB® code [1]. The postprocessing steps of the RLLSpec pipeline, which we will describe in the following paragraphs, were conducted for each of the five acquisition channels #DET1–#DET5 separately. For the sake of brevity, we will not distinguish between the individual acquisition channels in the notation of the postprocessed quantities. Depending on the available measurement data, the RLLSpec pipeline executes the following four steps or a subset thereof:

1. **Count Vector Aggregation** As a first step, the measured gross pulse-height spectra  $\mathbf{C}_{\text{gr},k} \in \mathbb{N}^{N_{\text{ch}} \times 1}$  and background pulse-height spectra  $\mathbf{C}_{\text{b},k} \in \mathbb{N}^{N_{\text{ch}} \times 1}$  with  $N_{\text{ch}} = 1024$  are summed over predefined sets  $\mathcal{D}_{\text{gr}} = \{k \in \mathbb{N}_+ \mid k \leq N_{\text{gr}}, N_{\text{gr}} \in \mathbb{N}_+\}$  and  $\mathcal{D}_{\text{b}} = \{k \in \mathbb{N}_+ \mid k \leq N_{\text{b}}, N_{\text{b}} \in \mathbb{N}_+\}$ , for which we may assume no or negligible variation in the experimental condition:

$$\mathbf{C}_{\text{gr}} = \sum_{k=1}^{N_{\text{gr}}} \mathbf{C}_{\text{gr},k} \quad (\text{S1a})$$

$$\mathbf{C}_{\text{b}} = \sum_{k=1}^{N_{\text{b}}} \mathbf{C}_{\text{b},k} \quad (\text{S1b})$$

where:

$\mathbf{C}_{\text{b}}$       background count vector  
 $\mathbf{C}_{\text{gr}}$      gross count vector

To minimize variation in the experimental conditions, the recorded pulse-height spectra from the far-field measurements in dynamic hover flight mode were filtered to include only those instances when the helicopter was aligned with the source on the ground at a predefined ground clearance (see Table S4). For the static near- and mid-field measurements, the source-detector setup remained unchanged between individual gross and background measurements.

2. **Count Rate Vector Computation** In a second step, dead-time corrected mean gross and background count rate pulse-height spectra are computed using the recorded live times  $t_{\text{gr}} = \sum_{k=1}^{N_{\text{gr}}} t_{\text{gr},k}$  and  $t_{\text{b}} = \sum_{k=1}^{N_{\text{b}}} t_{\text{b},k}$  and the aggregated count vectors from the first step:

$$\mathbf{c}_{\text{gr}} = \mathbf{C}_{\text{gr}}/t_{\text{gr}} \quad (\text{S2a})$$

$$\mathbf{c}_{\text{b}} = \mathbf{C}_{\text{b}}/t_{\text{b}} \quad (\text{S2b})$$

where:

|                          |                                  |                 |
|--------------------------|----------------------------------|-----------------|
| $\mathbf{c}_b$           | background count rate vector     | $\text{s}^{-1}$ |
| $\mathbf{c}_{\text{gr}}$ | gross count rate vector          | $\text{s}^{-1}$ |
| $t_b$                    | background measurement live time | $\text{s}$      |
| $t_{\text{gr}}$          | gross measurement live time      | $\text{s}$      |

The individual live times of the gross and background measurements conducted in this study are provided in the Tables S2–S4.

- 3. Background Correction** In a third step, dead-time and background corrected mean net count rate pulse-height spectra  $\mathbf{c}_{\text{net}} \in \mathbb{R}_+^{N_{\text{ch}} \times 1}$  are computed:

$$\mathbf{c}_{\text{net}} = \mathbf{c}_{\text{gr}} - \mathbf{c}_b \quad (\text{S3})$$

- 4. Spectral Signature Computation** If the source strength  $\xi$  of the adopted source during the gross measurement is known, the mean spectral signature can be computed by normalizing the mean net count rate pulse-height spectra in Eq. S3 by the corresponding source strength  $\xi$ :

$$\hat{\mathbf{c}}_{\text{exp}} = \mathbf{c}_{\text{net}} / \xi \quad (\text{S4})$$

with:

|                                 |                                  |                            |
|---------------------------------|----------------------------------|----------------------------|
| $\hat{\mathbf{c}}_{\text{exp}}$ | measured mean spectral signature | $\text{s}^{-1} [\xi]^{-1}$ |
| $\xi$                           | source strength                  | $[\xi]$                    |

In this study, the source strength  $\xi$  is parametrized by the known source activities  $\mathcal{A}$ , resulting in the measured mean spectral signature  $\hat{\mathbf{c}}_{\text{exp}}$  being expressed in units of  $\text{s}^{-1} \text{Bq}^{-1}$ . Note, that for the deployed radionuclide sources, we implicitly assume constant activities throughout the measurements. Given the short duration of the measurements relative to the radionuclides' half-lives, the effect of radioactive decay is negligible (cf. Sec. S1.4.1.4).

For all quantities discussed in this subsection, the RLLSpec pipeline provides uncertainty estimates. More information on these uncertainty estimates is provided in Sec. S1.4.1.

## S1.2 Calibration Pipeline: RLLCa1

For the Monte Carlo model presented in the main study, there are four main detector-specific meta-models with associated hyperparameters, which need to be derived from radiation measurements:

1. **Spectral energy calibration** Model relating the continuous pulse-height channel number  $\tilde{n}$  to the spectral energy  $E'$ .
2. **Spectral resolution calibration** A model to characterize the spectral resolution  $R_E$  as a function of the continuous pulse-height channel number  $\tilde{n}$ .
3. **LLD calibration** A model to account for the lower-level discriminator (LLD) at low spectral energies.
4. **NPSM calibration** A model to account for the non-proportional scintillation response of the NaI(Tl) crystals.

A dedicated pipeline, named RLLCa1, was developed using the MATLAB<sup>®</sup> code to infer the hyperparameters of these meta-models from radiation measurements. This pipeline is applied separately to each of the five acquisition channels #DET1–#DET5. Since the calibration of the adopted non-proportional scintillation model was already described in a previous work [2], we limit the discussion here to the conducted calibration of the first three meta-models.

### S1.2.1 Spectral Energy Calibration

As discussed in the main study, the Swiss AGRS system features automatic spectrum linearization with offset correction. As a result, a simple proportional energy calibration model has proven sufficient to characterize the spectral energy  $E'$  as a function of the continuous pulse-height channel number  $\tilde{n}$  for the specific acquisition channel:

$$E' = \Delta E' \tilde{n} \quad (\text{S5})$$

where:

|             |                                        |    |
|-------------|----------------------------------------|----|
| $E'$        | spectral energy                        | eV |
| $\Delta E'$ | spectral energy bin width              | eV |
| $\tilde{n}$ | continuous pulse-height channel number |    |

and with the continuous pulse-height channel number  $\tilde{n}$  being defined as a parameter that ranges continuously from 0.5 to  $N_{\text{ch}} + 0.5$  to align the integer channel numbers with the center of the pulse-height channels [1, 3].

The spectral energy bin width  $\Delta E'$  for each of the five acquisition channels can be calibrated by extracting centroids  $\mu_{\tilde{n}}$  of full energy peaks (FEPs) in measured net count rate spectra [3–5]. In this work, we selected an extensive set of FEPs to calibrate  $\Delta E'$ , covering a spectral range between  $\sim 122$  keV and  $\sim 2615$  keV (see Table S5). Gross and background measurements were conducted at the Calibration Laboratory at the Paul Scherrer Institute using dedicated radionuclide point sources and following the measurement protocols outlined by Breitenmoser et al. [6]. To derive the net count rate spectra from these radiation measurements, we applied the postprocessing pipeline RLLSpec described in Sec. S1.1. Similar to Breitenmoser et al. [6], we performed weighted linear least-squares (WLLS) regression using Gaussian singlet and

multiplet peak models combined with a physics-oriented empirical baseline correction [7, 8] to retrieve the centroids  $\mu_{\tilde{n}}$  from the measured FEPs:

$$c_{\text{net}}(\tilde{n}) = c_{\text{bl}}(\tilde{n}) + \sum_{i=1}^{N_{\text{FEP}}} z_i \exp \left[ -\frac{(\tilde{n} - \mu_{\tilde{n},i})^2}{2\sigma_{\tilde{n},i}^2} \right] \quad (\text{S6})$$

where:

|                      |                               |                 |
|----------------------|-------------------------------|-----------------|
| $z$                  | normalization parameter       | $\text{s}^{-1}$ |
| $c_{\text{net}}$     | net count rate                | $\text{s}^{-1}$ |
| $c_{\text{bl}}$      | baseline count rate           | $\text{s}^{-1}$ |
| $N_{\text{FEP}}$     | number of FEPs                |                 |
| $\mu_{\tilde{n}}$    | mean of the FEP               |                 |
| $\sigma_{\tilde{n}}$ | standard deviation of the FEP |                 |

Utilizing the obtained set of centroids  $\mu_{\tilde{n}}$  and related photon emission energies (see Table S5), we then retrieved the spectral energy bin width  $\Delta E'$  for each acquisition channel by performing WLLS regression for the proportional energy calibration model given by Eq. S5. The calibrated spectral energy bin widths and associated uncertainties are listed in Table S6. The derived energy calibration models are displayed in Fig. S1.



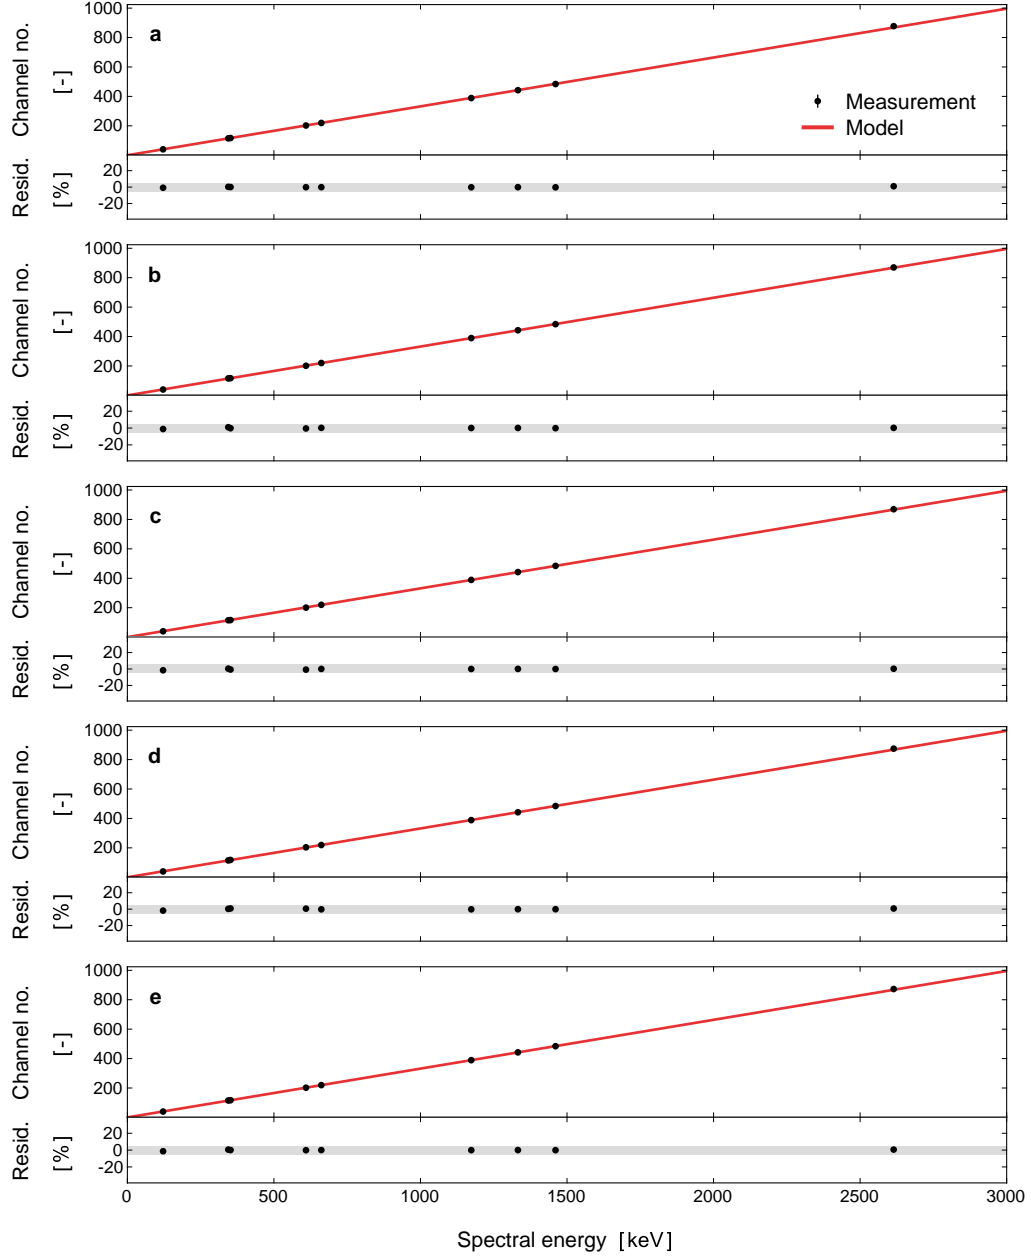

**Figure S1 Energy calibration models.** Here, we present derived energy calibration models relating the spectral energy  $E'$  to the continuous pulse-height channel number  $\tilde{n}$  for the five acquisition channels #DET1–#DET5 (a–e). Measurement uncertainties are provided as 1 standard deviation (SD) error bars (hidden by the marker size). The model uncertainty is characterized by 99 % prediction intervals displayed as red-shaded areas (hidden by the line width). In addition, the relative residuals (Resid., normalized by the mean measured values) are provided for each acquisition channel with the 5 % band highlighted.

### S1.2.2 Spectral Resolution Calibration

Similar to previous studies [2, 6, 9–13], we parametrize the spectral resolution  $R_E$  as a function of the continuous pulse-height channel number  $\tilde{n}$  using an empirical power-law model:

$$R_E(\tilde{n}) = a_1 \tilde{n}^{a_2} \quad (\text{S7})$$

with:

$a_1$       scale coefficient  
 $a_2$       power coefficient

The spectral resolution of inorganic scintillators is commonly quantified as the full width at half maximum (FWHM) of a FEP in the pulse-height spectrum divided by the FEP's centroid [4]:

$$R_E = \frac{\text{FWHM}(\mu_{\tilde{n}})}{\mu_{\tilde{n}}} \quad (\text{S8})$$

where:

FWHM      full width at half maximum of the FEP  
 $\mu_{\tilde{n}}$       centroid of the FEP

Both the centroids  $\mu_{\tilde{n}}$  and the FWHMs can be retrieved from the radiation measurements described in Sec. S1.2.1, with the centroids being equivalent to the means of the FEPs and by exploiting the analytical relation  $\text{FWHM} = 2\sqrt{2\log 2} \sigma_{\tilde{n}}$  for the dispersion of Gaussian distributions [4]. Using this calibration data, we then estimated the scale and power coefficients in Eq. S7 for each acquisition channel using again WLLS regression. The derived coefficients and associated uncertainties are listed in Table S6. The calibrated resolution models are displayed in Fig. S2.

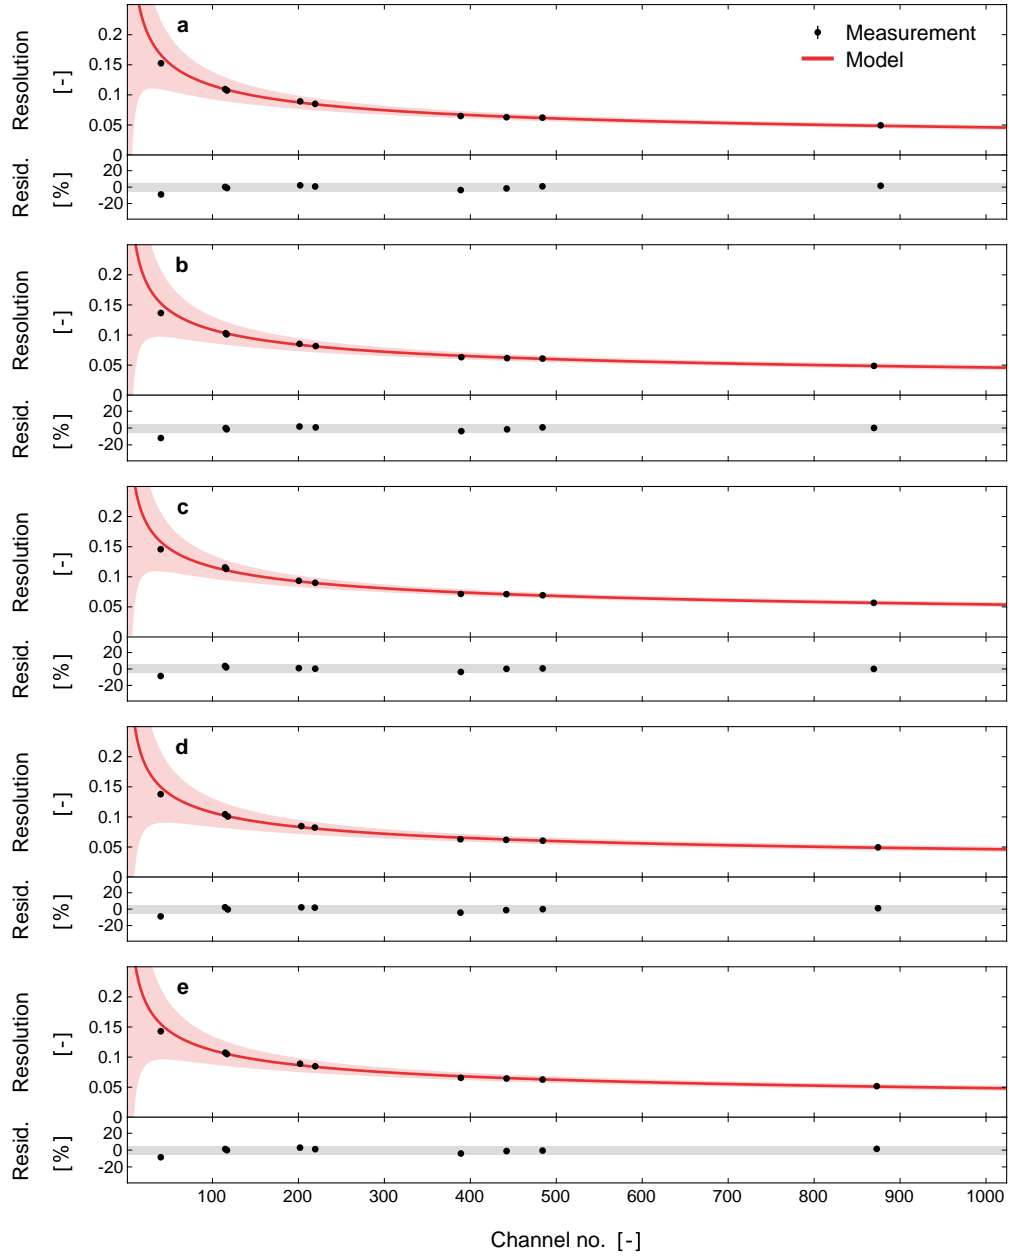

**Figure S2 Spectral resolution models.** Here, we present derived spectral resolution models relating the continuous pulse-height channel number  $\tilde{n}$  to the spectral resolution  $R_E$  for the five acquisition channels #DET1-#DET5 (a-e). Measurement uncertainties are provided as 1 standard deviation (SD) error bars (hidden by the marker size). The model uncertainty is characterized by 99% prediction intervals displayed as red-shaded areas. In addition, the relative residuals (Resid., normalized by the mean measured values) are provided for each acquisition channel with the 5% band highlighted.

### S1.2.3 LLD Calibration

As in our previous work [2, 6], we adopt a heuristic Gaussian model to correct for the lower-level discriminator (LLD) in the simulated spectral signatures:

$$\hat{c}_{w/LLD,n} = \hat{c}_{w/oLLD,n} \Phi\left(\frac{n - \mu_{LLD}}{\sigma_{LLD}}\right) \quad (S9)$$

where:

|                    |                                              |                          |
|--------------------|----------------------------------------------|--------------------------|
| $\hat{c}_{w/LLD}$  | mean spectral signature with LLD             | $s^{-1} \text{ Bq}^{-1}$ |
| $\hat{c}_{w/oLLD}$ | mean spectral signature without LLD          | $s^{-1} \text{ Bq}^{-1}$ |
| $n$                | pulse-height channel number                  |                          |
| $\mu_{LLD}$        | mean lower-level discriminator               |                          |
| $\sigma_{LLD}$     | lower-level discriminator standard deviation |                          |

and with  $\Phi(\cdot)$  denoting the standard normal cumulative distribution function. This heuristic model is motivated by the idea that the fixed lower-level discriminator  $\mathcal{H}_{\min}$  is fluctuating due to inherent noise in the photomultiplier tubes, multichannel analyzers, and associated electronics resulting in an approximately normally distributed cut-off with the mean  $\mu_{LLD}$  corresponding to the predefined LLD threshold and a standard deviation  $\sigma_{LLD}$  determined by the level of noise.

The model parameters,  $\mu_{LLD}$  and  $\sigma_{LLD}$ , were calibrated for each of the five acquisition channels #DET1–#DET5 using the measured and simulated spectral signatures of a  $^{60}\text{Co}$  radionuclide point source from our calibration dataset (cf. Table S5). Specifically, we optimized the model parameters based on the  $\chi^2$ -objective function to align the simulated spectral signatures with the measured ones:

$$(\hat{\mu}_{LLD}, \hat{\sigma}_{LLD}) = \arg \min_{\mu_{LLD}, \sigma_{LLD}} \chi^2 \quad (S10)$$

with  $\hat{\mu}_{LLD}$  and  $\hat{\sigma}_{LLD}$  representing the arguments of the global  $\chi^2$ -minimum. The  $\chi^2$ -objective function was defined as:

$$\chi^2 = \frac{1}{N_{\text{ch}}^* - 2} \sum_{n=1}^{N_{\text{ch}}^*} \frac{(\hat{c}_{\text{exp},n} - \hat{c}_{\text{sim},n}(\mu_{LLD}, \sigma_{LLD}))^2}{\hat{\sigma}_{\text{exp},n}^2 + \hat{\sigma}_{\text{sim},n}^2} \quad (S11)$$

where:

|                             |                                                 |                          |
|-----------------------------|-------------------------------------------------|--------------------------|
| $\hat{c}_{\text{exp}}$      | measured mean spectral signature                | $s^{-1} \text{ Bq}^{-1}$ |
| $\hat{c}_{\text{sim}}$      | simulated mean spectral signature               | $s^{-1} \text{ Bq}^{-1}$ |
| $N_{\text{ch}}^*$           | reduced number of pulse-height channels         |                          |
| $n$                         | pulse-height channel number                     |                          |
| $\hat{\sigma}_{\text{exp}}$ | measured spectral signature standard deviation  | $s^{-1} \text{ Bq}^{-1}$ |
| $\hat{\sigma}_{\text{sim}}$ | simulated spectral signature standard deviation | $s^{-1} \text{ Bq}^{-1}$ |

with  $\hat{c}_{\text{exp}}$  and  $\hat{\sigma}_{\text{exp}}$  obtained by the RLLSpec pipeline (cf. Sec. S1.1) and  $\hat{c}_{\text{sim}}$  and  $\hat{\sigma}_{\text{sim}}$  obtained by the NPScinMC pipeline (cf. Sec. S1.3). We solved the global minimization problem in Eq. S10 by the radial basis surrogate solver `surrogateopt` [14, 15] using the MATLAB<sup>®</sup> code. The spectral range was restricted to  $n \leq \lfloor 50 \text{ keV}/\Delta E' \rfloor = N_{\text{ch}}^*$  with  $\{\mu_{LLD} \in \mathbb{R}_+ \mid \mu_{LLD} \leq 30 \text{ keV}/\Delta E'\}$  and  $\{\sigma_{LLD} \in \mathbb{R}_+ \mid 0.1 \text{ keV}/\Delta E' \leq \sigma_{LLD} \leq 20 \text{ keV}/\Delta E'\}$ .

The resulting  $\chi^2$ -contour maps for the five acquisition channels are presented in Fig. S3. For each acquisition channel, the radial basis surrogate solver converged to a global minimum  $\chi^2_{\min}$  indicated by a plus sign in the individual contour maps. Confidence limits are illustrated adopting 1 and 2 standard deviation contour lines [16]. Depending on the acquisition channel, the mean lower-level discriminator is found to be between  $\sim 15$  keV and  $\sim 20$  keV with a standard deviation between  $\sim 3$  keV and  $\sim 6$  keV. The derived model parameters are also listed in Table S6.

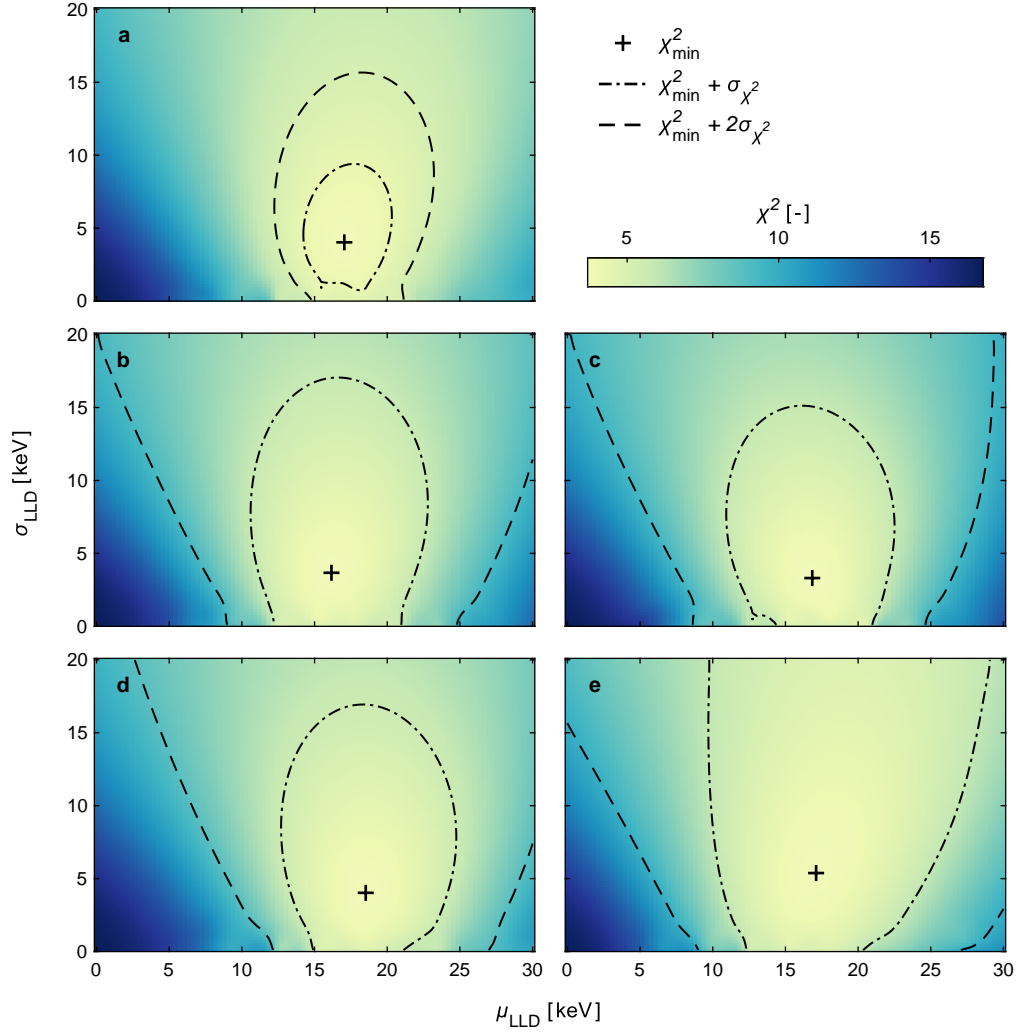

**Figure S3  $\chi^2$ -contour maps of the lower-level discriminator model parameters.** Here, the results of the LLD calibration are presented as  $\chi^2$ -contour maps of the lower-level discriminator model parameters  $\mu_{\text{LLD}}$  and  $\sigma_{\text{LLD}}$  for the the sum acquisition channel #DET5 (a) as well as for the four individual channels #DET1-#DET4 (b-e). The global minima  $\chi^2_{\text{min}}$  are marked with a plus sign together with the corresponding 1-sigma and 2-sigma confidence regions indicated by the dashed-dotted and dashed contour lines, respectively. For the reader's convenience, the unit of the lower-level discriminator model parameters  $\mu_{\text{LLD}}$  and  $\sigma_{\text{LLD}}$  was converted from continuous pulse-height channel numbers to spectral energies using the energy calibration models derived by the RLLCa1 pipeline (cf. Sec. S1.2.1).

### S1.3 Postprocessing Pipeline: NPScinMC

Similar to the postprocessing of the measurement data, a dedicated pipeline named NPScinMC was developed using the MATLAB<sup>®</sup> code to postprocess the simulation data obtained by online Non-proportional Scintillation Monte Carlo (NPSMC) [1, 2], that is the set of scaled energy deposition events  $E_{\text{dep},i}\eta_{\text{cap},i}$  with  $\{i \in \mathbb{N}_+ \mid i \leq N_{\text{dep}}, N_{\text{dep}} \in \mathbb{N}_+\}$  for each of the four scintillation crystals and with  $N_{\text{dep}}$  being the number of scored events for a predefined number of Monte Carlo primaries  $N_{\text{pr}} \in \mathbb{N}_+$  with  $N_{\text{pr}} \geq N_{\text{dep}}$ . The scaling with the energy transfer efficiency  $\eta_{\text{cap}}$  is performed online during the NPSMC simulations using a non-proportional scintillation model proposed by Payne et al. [17, 18], as described in detail in our previous work [1, 2].

The NPScinMC pipeline is applied to each of the four single acquisition channels #DET1–#DET4 separately. The fifth acquisition channel #DET5 is obtained by summing the derived pulse-height spectra of the four individual single acquisition channels. Consequently, only the calibration models for the four single acquisition channels are used in the postprocessing of the simulation data. The NPScinMC pipeline reconstructs the spectral signature for a given set of scaled energy deposition events in a given acquisition channel in four distinct steps:

1. **Pulse-Height Channel Conversion** In a first step, the scaled deposited energies  $E_{\text{dep},i}\eta_{\text{cap},i}$  are transformed to continuous pulse-height channel numbers  $\tilde{n}_{\text{dep}}^* \in \mathbb{R}_+$ :

$$\tilde{n}_{\text{dep},i}^* = \frac{f_{\text{np}}(E_{\text{dep},i}\eta_{\text{cap},i})}{\Delta E'} \quad (\text{S12})$$

where:

|                            |                                                                          |    |
|----------------------------|--------------------------------------------------------------------------|----|
| $E_{\text{dep}}$           | deposited energy                                                         | eV |
| $\Delta E'$                | spectral energy bin width                                                | eV |
| $\tilde{n}_{\text{dep}}^*$ | continuous raw pulse-height channel number of an energy deposition event |    |
| $\eta_{\text{cap}}$        | energy transfer efficiency                                               |    |

with the spectral energy bin width  $\Delta E'$  being derived by the RLLCa1 pipeline (cf. Sec. S1.2.1). The non-proportional scintillation scaling function  $f_{\text{np}}(\cdot)$  is based on a modified Akima spline interpolation model [19] and was calibrated by NPSMC in a previous studies [2].

2. **Broadening & Binning** In the second step, to account for the finite detector resolution, the converted individual energy deposition events  $\tilde{n}_{\text{dep},i}^*$  are convoluted with the spectral resolution models calibrated by the RLLCa1 pipeline (see Sec. S1.2.2). Like in previous studies [10, 11, 13, 20–30], the random continuous pulse-height channel number of energy deposition events  $\tilde{\mathfrak{n}}_{\text{dep}}$  are assumed to be normally distributed:

$$\tilde{\mathfrak{n}}_{\text{dep}} \sim \mathcal{N}\left(\tilde{n}_{\text{dep}} \mid \tilde{n}_{\text{dep}}^*, \sigma_{\tilde{n}}'^2(\tilde{n}_{\text{dep}}^*)\right) \quad (\text{S13})$$

with a mean equal to the simulated raw energy deposition  $\tilde{n}_{\text{dep}}^*$  obtained by Eq. S12 and a standard deviation  $\sigma_{\tilde{n}}'$  estimated by:

$$\sigma_{\tilde{n}}'(\tilde{n}_{\text{dep}}^*) = \sqrt{\sigma_{\tilde{n}}^2(\tilde{n}_{\text{dep}}^*) - \sigma_{\tilde{n},\text{intr}}^2(\tilde{n}_{\text{dep}}^*)} \quad (\text{S14})$$

where:

|                                  |                                                                          |
|----------------------------------|--------------------------------------------------------------------------|
| $\tilde{n}_{\text{dep}}^*$       | continuous raw pulse-height channel number of an energy deposition event |
| $\sigma_{\tilde{n}}$             | spectral resolution standard deviation                                   |
| $\sigma_{\tilde{n},\text{intr}}$ | spectral intrinsic resolution standard deviation                         |

Given that the scaled energy deposition events  $E_{\text{dep}}\eta_{\text{cap}}$  resulting from online NPSMC are intrinsically broadened, the spectral resolution standard deviation  $\sigma_{\tilde{n}}$  is reduced in quadrature by the intrinsic spectral resolution standard deviation  $\sigma_{\tilde{n},\text{intr}}$  in Eq. S14. To model the complex non-linear behavior of  $\sigma_{\tilde{n},\text{intr}}$ , we calibrated a Gaussian process regression model [31] in our previous work [1, 2]. The spectral resolution standard deviation  $\sigma_{\tilde{n}}$  is derived by the RLLCa1 pipeline (cf. Sec. S1.2.2).

The convolution, sometimes also referred to as Gaussian broadening [20, 23, 24, 29, 30], is performed in parallel with the binning of the simulated energy deposition events  $\tilde{n}_{\text{dep},i}^*$  to generate the simulated mean number of scintillation pulses  $C_n$  in pulse-height channel  $n$  with  $\{n \in \mathbb{N}_+ \mid n \leq N_{\text{ch}}, N_{\text{ch}} \in \mathbb{N}_+\}$ :

$$C_n = \sum_{i=1}^{N_{\text{dep}}} \int_{n-\frac{1}{2}}^{n+\frac{1}{2}} \frac{1}{\sigma'_{\tilde{n}}(\tilde{n}_{\text{dep},i}^*)} \varphi\left(\frac{\tilde{n} - \tilde{n}_{\text{dep},i}^*}{\sigma'_{\tilde{n}}(\tilde{n}_{\text{dep},i}^*)}\right) d\tilde{n} \quad (\text{S15a})$$

$$= \sum_{i=1}^{N_{\text{dep}}} \Phi\left(\frac{n + \frac{1}{2} - \tilde{n}_{\text{dep},i}^*}{\sigma'_{\tilde{n}}(\tilde{n}_{\text{dep},i}^*)}\right) - \Phi\left(\frac{n - \frac{1}{2} - \tilde{n}_{\text{dep},i}^*}{\sigma'_{\tilde{n}}(\tilde{n}_{\text{dep},i}^*)}\right) \quad (\text{S15b})$$

where we use  $\varphi(\cdot)$  and  $\Phi(\cdot)$  to denote the standard normal probability density function and standard normal cumulative distribution function, respectively. For the spectrometer used in the present work, the number of pulse-height channels  $N_{\text{ch}}$  is fixed to 1024.

Considering that typical high-fidelity simulations require  $N_{\text{dep}} \geq 10^5$ , sequential summation of the individual energy deposition events in Eqs. S15a and S15b is computationally inefficient, in particular, if the convolution is performed multiple times for identical energy deposition events. Therefore, we apply a modified discrete convolution operation in NPSMC by discretizing the continuous  $\tilde{n}$  domain introducing refined pulse-height channel numbers  $\tilde{n}_j^+ = (j-1)\Delta\tilde{n}^+$  with refined bin width  $\Delta\tilde{n}^+$  and index  $\{j \in \mathbb{N}_+ \mid j \leq N_{\text{ch}}^+, N_{\text{ch}}^+ \in \mathbb{N}_+\}$ . To cover the full spectral domain, the number of refined bins  $N_{\text{ch}}^+$  are constrained to  $N_{\text{ch}}^+ > N_{\text{ch}}/\Delta\tilde{n}^+$ . In this work, a refined bin width of  $\Delta\tilde{n}^+ = 10^{-1}$  and  $N_{\text{ch}}^+ = (N_{\text{ch}} + 30)/\Delta\tilde{n}^+$  was applied. Using this discretization scheme, we can rewrite Eq. S15b in matrix form as follows:

$$\mathbf{C} = \mathbf{G}\mathbf{C}^+ \quad (\text{S16})$$

where:

|                |                        |
|----------------|------------------------|
| $\mathbf{C}$   | mean count vector      |
| $\mathbf{C}^+$ | prebinned count vector |
| $\mathbf{G}$   | Gaussian weight matrix |



As the name implies,  $\mathbf{C} \in \mathbb{R}_+^{N_{\text{ch}} \times 1}$  represents the mean number of energy deposition events in the individual pulse-height channels. In contrast,  $\mathbf{C}^+ \in \mathbb{N}^{N_{\text{ch}}^+ \times 1}$  denotes the prebinned count vector of the simulated energy deposition events using the refined pulse-height channel numbers  $\tilde{n}^+$ , i.e. the number of simulated energy deposition events in each refined pulse-height channel  $j$  binned by  $\tilde{n}_j^+ - \Delta\tilde{n}^+/2 < \tilde{n}_{\text{dep}}^* \leq \tilde{n}_j^+ + \Delta\tilde{n}^+/2$ . The elements of the Gaussian weight matrix  $\mathbf{G}$  are computed as follows:

$$G_{n,j} = \Phi\left(\frac{n + \frac{1}{2} - \tilde{n}_j^+}{\sigma'_{\tilde{n}}(\tilde{n}_j^+)}\right) - \Phi\left(\frac{n - \frac{1}{2} - \tilde{n}_j^+}{\sigma'_{\tilde{n}}(\tilde{n}_j^+)}\right) \quad (\text{S17})$$

with the index  $\{j \in \mathbb{N}_+ \mid j \leq N_{\text{ch}}^+, N_{\text{ch}}^+ \in \mathbb{N}_+\}$  of the newly introduced refined pulse-height channel number  $\tilde{n}^+$  and the (original) pulse-height channel number  $\{n \in \mathbb{N}_+ \mid n \leq N_{\text{ch}}, N_{\text{ch}} = 1024\}$ , giving a weight matrix  $\mathbf{G} \in \mathbb{R}_+^{N_{\text{ch}} \times N_{\text{ch}}^+}$ .

Using the matrix form in Eq. S16 and the outlined discretization scheme, the computational efficiency of the numerical convolution operation can be improved by a factor  $> \mathcal{O}(10^2)$  with discretization errors kept below  $<1\%$  in the spectral domain of interest  $\mathcal{D}_{\text{SDOI}}$  (cf. Fig. S8). The spectral domain of interest  $\mathcal{D}_{\text{SDOI}}$  is defined as the spectral band with continuous pulse-height channel numbers  $\{\tilde{n} \in \mathbb{R}_+ \mid \mu_{\text{LLD}} + 2\sigma_{\text{LLD}} \leq \tilde{n} \leq \min(\{\max(E_\gamma)/\Delta E' + 2\sigma_{\tilde{n}}, N_{\text{ch}} + \frac{1}{2}\})\}$ . Here,  $\max(E_\gamma)$  represents the maximum photon source energy,  $\Delta E'$  the constant spectral energy bin width and  $\sigma_{\tilde{n}}$  the standard deviation of the associated FEP in the pulse-height spectrum. For practical reasons, only emissions with a relative photon intensity  $I_\gamma$  over  $1\%$  are considered for radionuclide sources. The lower limit of  $\mathcal{D}_{\text{SDOI}}$  is defined by the mean continuous pulse-height channel number  $\mu_{\text{LLD}}$  and standard deviation  $\sigma_{\text{LLD}}$  associated with the LLD in the given pulse-height spectrum (cf. Sec. S1.2.3).

- 3. Normalization** To obtain spectral signature estimates, the mean count vector  $\mathbf{C}$  of the previous step needs to be normalized by the integrated source strength  $\Xi$ :

$$\hat{\mathbf{c}}_{\text{sim}} = \mathbf{C} \Xi^{-1} \quad (\text{S18})$$

where:

|                                 |                                   |                    |
|---------------------------------|-----------------------------------|--------------------|
| $\Xi$                           | integrated source strength        | $[\xi]s$           |
| $\mathbf{C}$                    | mean count vector                 |                    |
| $\hat{\mathbf{c}}_{\text{sim}}$ | simulated mean spectral signature | $s^{-1}[\xi]^{-1}$ |

The integrated source strength  $\Xi$  is defined as:

$$\Xi = \int_{\Delta t} \xi \, dt \quad (\text{S19})$$

with:

|       |                 |         |
|-------|-----------------|---------|
| $\xi$ | source strength | $[\xi]$ |
|-------|-----------------|---------|

In Monte Carlo radiation transport simulations,  $\Xi$  is equivalent to the number of primaries  $N_{\text{pr}}$ , that is the number of simulated source histories, normalized by a source specific factor  $F_{\text{src}}$  characterizing the detailed source geometry and/or the source matter:

$$\Xi = N_{\text{pr}} F_{\text{src}}^{-1} \quad (\text{S20})$$

with:

|                  |                               |                    |
|------------------|-------------------------------|--------------------|
| $F_{\text{src}}$ | source geometry-matter factor | $[F_{\text{src}}]$ |
| $N_{\text{pr}}$  | number of primaries           |                    |

Here, we list commonly used source geometry-matter factors for several prominent homogeneous radionuclide sources typically employed in Monte Carlo simulations, along with the corresponding units for the simulated mean spectral signatures:

$$F_{\text{src}} = \begin{cases} 1 & [\hat{\mathbf{c}}_{\text{sim}}] = \frac{1}{\text{s Bq}} & \text{point source} & (\text{S21a}) \\ A_{\text{src}} & [\hat{\mathbf{c}}_{\text{sim}}] = \frac{\text{m}^2}{\text{s Bq}} & \text{surface source} & (\text{S21b}) \\ V_{\text{src}} & [\hat{\mathbf{c}}_{\text{sim}}] = \frac{\text{m}^3}{\text{s Bq}} & \text{atmospheric volume source} & (\text{S21c}) \\ V_{\text{src}} \rho_{\text{src}} & [\hat{\mathbf{c}}_{\text{sim}}] = \frac{\text{kg}}{\text{s Bq}} & \text{terrestrial volume source} & (\text{S21d}) \end{cases}$$

where:

|                     |                     |                    |
|---------------------|---------------------|--------------------|
| $A_{\text{src}}$    | source area         | $\text{m}^2$       |
| $V_{\text{src}}$    | source volume       | $\text{m}^3$       |
| $\rho_{\text{src}}$ | source mass density | $\text{kg m}^{-3}$ |

In this work, we exclusively adopt radionuclide point sources. Accordingly, we set  $F_{\text{src}} = 1$  with  $[\hat{\mathbf{c}}_{\text{sim}}] = \text{s}^{-1} \text{Bq}^{-1}$ , ensuring consistency with the dimensions of the measured mean spectral signature estimate,  $\hat{\mathbf{c}}_{\text{exp}}$ , as obtained from the RLLSpec pipeline (cf. Sec. S1.1).

- 4. LLD Correction** As a last step in the NPScinMC pipeline, the simulated mean spectral signature  $\hat{\mathbf{c}}_{\text{sim}}$  estimated by Eq. S18 is corrected for the LLD using a heuristic Gaussian model discussed in Sec. S1.2.3:

$$\hat{\mathbf{c}}_{\text{sim,w/LLD},n} = \hat{\mathbf{c}}_{\text{sim},n} \Phi\left(\frac{n - \mu_{\text{LLD}}}{\sigma_{\text{LLD}}}\right) \quad (\text{S22})$$

where:

|                                 |                                              |                            |
|---------------------------------|----------------------------------------------|----------------------------|
| $\hat{\mathbf{c}}_{\text{sim}}$ | simulated mean spectral signature element    | $\text{s}^{-1} [\xi]^{-1}$ |
| $n$                             | pulse-height channel number                  |                            |
| $\mu_{\text{LLD}}$              | mean lower-level discriminator               |                            |
| $\sigma_{\text{LLD}}$           | lower-level discriminator standard deviation |                            |

and with  $\Phi(\cdot)$  denoting again the standard normal cumulative distribution function. The model-specific parameters in Eq. S22, i.e.  $\mu_{\text{LLD}}$  and  $\sigma_{\text{LLD}}$ , are calibrated for the four acquisition channels #DET1–#DET4 by the RLLCa1 pipeline (see Sec. S1.2.2). For notational convenience, the mean spectral signature including the LLD model  $\hat{\mathbf{c}}_{\text{sim,LLD}}$  will be denoted by  $\hat{\mathbf{c}}_{\text{sim}}$  in the main study.

Like for the RLLSpec pipeline, the NPScinMC pipeline provides also uncertainty estimates for the derived quantities presented in this section. More information on these uncertainty estimates is provided in Sec. S1.4.2.

## S1.4 Uncertainty Quantification

The spectral quantities derived by the postprocessing pipelines RLLSpec and NPScinMC discussed in Secs. S1.1 and S1.3 are inherently subject to uncertainties. In this section, we will briefly discuss the uncertainty analysis for these spectral quantities. In line with the standard established by the Joint Committee for Guides in Metrology [32], we will distinguish between two main categories of uncertainties. The first category is associated with all uncertainties that are estimated by an observed frequency distribution (simulated or measured). This is known as type A [5, 32], aleatory [33–35], or statistical uncertainty [36–38]. The second category encompasses all uncertainties derived from sources other than observed frequency distributions, such as literature sources, calibration certificates, or expert knowledge. This is known as type B [5, 32], epistemic [33–35], or systematic uncertainty [36–38]. We will use the terms "statistical" and "systematic" in this work to refer to these two categories of uncertainty, respectively.

### S1.4.1 Measurement Uncertainty

Uncertainty quantification in radiation measurements is extensively addressed in the literature [4, 5, 39] and standardized by the International Organization for Standardization (ISO) in ISO 11929. In this work, we adopt the uncertainty analysis methodology for radiation measurements detailed by Knoll [4].

#### S1.4.1.1 Statistical Measurement Uncertainty

For the radiation measurements, the statistical uncertainty of the spectral quantities discussed in Sec. S1.1 are characterized by the standard deviation and estimated by a probabilistic Poisson model according to Knoll [4]:

$$\sigma_{C_{\text{gr}}} = (C_{\text{gr}})^{\circ \frac{1}{2}} \quad (\text{S23a})$$

$$\sigma_{C_{\text{b}}} = (C_{\text{b}})^{\circ \frac{1}{2}} \quad (\text{S23b})$$

$$\sigma_{c_{\text{gr}}} = (C_{\text{gr}})^{\circ \frac{1}{2}} / t_{\text{gr}} \quad (\text{S23c})$$

$$\sigma_{c_{\text{b}}} = (C_{\text{b}})^{\circ \frac{1}{2}} / t_{\text{b}} \quad (\text{S23d})$$

$$\sigma_{c_{\text{net}}} = \left( C_{\text{gr}} / t_{\text{gr}}^2 + C_{\text{b}} / t_{\text{b}}^2 \right)^{\circ \frac{1}{2}} \quad (\text{S23e})$$

where:

|                 |                                  |   |
|-----------------|----------------------------------|---|
| $C_{\text{b}}$  | background count vector          |   |
| $C_{\text{gr}}$ | gross count vector               |   |
| $t_{\text{b}}$  | background measurement live time | s |
| $t_{\text{gr}}$ | gross measurement live time      | s |

and with  $\circ$  being defined as the Hadamard or element-wise power. By combining Eqs. S4 and S23e, we may estimate the statistical uncertainty in the measured mean spectral signature  $\hat{c}_{\text{exp}}$  for a given radionuclide source with activity  $\mathcal{A}$  at measurement start time as [4]:

$$\hat{\sigma}_{\text{exp,stat}} = \mathcal{A}^{-1} \sigma_{c_{\text{net}}} \quad (\text{S24a})$$

$$= \mathcal{A}^{-1} \left( \mathbf{C}_{\text{gr}}/t_{\text{gr}}^2 + \mathbf{C}_{\text{b}}/t_{\text{b}}^2 \right)^{\frac{1}{2}} \quad (\text{S24b})$$

where:

|                           |                                           |                 |
|---------------------------|-------------------------------------------|-----------------|
| $\mathcal{A}$             | source activity at measurement start time | Bq              |
| $\sigma_{c_{\text{net}}}$ | net standard deviation count rate vector  | $\text{s}^{-1}$ |

#### S1.4.1.2 Systematic Measurement Uncertainty

The measured mean spectral signature  $\hat{\mathbf{c}}_{\text{exp}}$  is subject to both statistical and systematic uncertainties. Here, we limit the quantification of the systematic uncertainty to that introduced by scaling  $\hat{\mathbf{c}}_{\text{exp}}$  with the source strength  $\xi$ , which is anticipated to be the largest source of systematic uncertainty for the radiation measurements conducted in this work. In case of a radionuclide source, we may estimate the systematic uncertainty in the measured mean spectral signature  $\hat{\mathbf{c}}_{\text{exp}}$  by applying the standard error propagation methodology for independent variables [32, 37, 41] to Eq. S4, resulting in:

$$\hat{\sigma}_{\text{exp,sys}} = \mathbf{c}_{\text{net}} \sigma_{\mathcal{A}} \mathcal{A}^{-2} \quad (\text{S25})$$

where:

|                           |                                               |                 |
|---------------------------|-----------------------------------------------|-----------------|
| $\mathcal{A}$             | source activity at measurement start time $t$ | Bq              |
| $\sigma_{\mathcal{A}}$    | activity standard deviation                   | Bq              |
| $\mathbf{c}_{\text{net}}$ | net count rate vector                         | $\text{s}^{-1}$ |

For a calibration radionuclide source with a single decay channel and stable progeny, we may estimate the activity of the given radionuclide as a function of time  $t$  by the exponential decay law [4]:

$$\mathcal{A}(t) = \mathcal{A}_0 \exp \left[ -\frac{\log(2)\Delta t}{t_{1/2}} \right] \quad (\text{S26})$$

where:

|                 |                                         |    |
|-----------------|-----------------------------------------|----|
| $\mathcal{A}_0$ | source activity at reference date $t_0$ | Bq |
| $t_{1/2}$       | half-life                               | s  |

and with  $\Delta t$  being defined as the difference  $\Delta t = t - t_0$  between the time  $t$  and the reference date  $t_0$ . Consequently, we estimate the activity standard deviation  $\sigma_{\mathcal{A}}$  using again the standard error propagation methodology for independent variables [32, 37, 41] applied to Eq. S26 with the three independent variables, that are the reference activity  $\mathcal{A}_0$  at  $t_0$ , the half-life  $t_{1/2}$  as well as the time difference  $\Delta t$  [1]:

$$\sigma_{\mathcal{A}} = \mathcal{A} \sqrt{\left( \frac{\sigma_{\mathcal{A}_0}}{\mathcal{A}_0} \right)^2 + \left( \frac{\log(2)\Delta t \sigma_{t_{1/2}}}{t_{1/2}^2} \right)^2 + \left( \frac{\log(2)\sigma_{\Delta t}}{t_{1/2}} \right)^2} \quad (\text{S27})$$

where:

|                          |                                                                                                                      |    |
|--------------------------|----------------------------------------------------------------------------------------------------------------------|----|
| $\mathcal{A}$            | source activity at measurement start time $t$                                                                        | Bq |
| $\mathcal{A}_0$          | source activity at reference date $t_0$                                                                              | Bq |
| $t_{1/2}$                | half-life                                                                                                            | s  |
| $\sigma_{\mathcal{A}_0}$ | reference activity standard deviation                                                                                | Bq |
| $\sigma_{t_{1/2}}$       | half-life standard deviation                                                                                         | s  |
| $\sigma_{\Delta t}$      | standard deviation in the time difference between the reference date $t_0$ and the start time $t$ of the measurement | s  |

For all radiation sources used in this work, the relative contribution of the uncertainty in  $\sigma_{t_{1/2}}$  and  $\sigma_{\Delta t}$  to the total uncertainty in  $\mathcal{A}$  is found to be smaller than 1 %.

#### S1.4.1.3 Combined Measurement Uncertainty

The combined uncertainty in the measured spectral signature  $\hat{\mathbf{c}}_{\text{exp}}$  is estimated by combining the related statistical and systematic uncertainties in quadrature as suggested by the Particle Data Group et al. [36] and the Joint Committee for Guides in Metrology [32]:

$$\hat{\sigma}_{\text{exp}} = \left( \hat{\sigma}_{\text{exp,stat}}^{\circ 2} + \hat{\sigma}_{\text{exp,sys}}^{\circ 2} \right)^{\circ \frac{1}{2}} \quad (\text{S28a})$$

$$= \hat{\mathbf{c}}_{\text{exp}} \odot \left[ \left( \sigma_{\mathbf{c}_{\text{net}}} \oslash \mathbf{c}_{\text{net}} \right)^{\circ 2} + \left( \frac{\sigma_{\mathcal{A}}}{\mathcal{A}} \right)^2 \mathbf{J}_{N_{\text{ch}},1} \right]^{\circ \frac{1}{2}} \quad (\text{S28b})$$

where:

|                                  |                                                            |                                |
|----------------------------------|------------------------------------------------------------|--------------------------------|
| $\hat{\sigma}_{\text{exp,stat}}$ | measured statistical spectral signature standard deviation | $\text{s}^{-1} \text{Bq}^{-1}$ |
| $\hat{\sigma}_{\text{exp,sys}}$  | measured systematic spectral signature standard deviation  | $\text{s}^{-1} \text{Bq}^{-1}$ |

and with  $\odot$  and  $\oslash$  denoting the Hadamard, i.e. element-wise, product and division, respectively. The all-ones matrix  $\mathbf{J}_{m,n}$  is defined as a matrix of ones with dimension  $m \times n$ .

In this work,  $\hat{\sigma}_{\text{exp}}$  is indicated in each figure that presents measured spectral signatures  $\hat{\mathbf{c}}_{\text{exp}}$ . If applicable, the coefficient of variation vector  $\mathbf{CV}_{\text{exp}} \in \mathbb{R}_+^{N_{\text{ch}} \times 1}$  defined as:

$$\mathbf{CV}_{\text{exp}} = \hat{\sigma}_{\text{exp}} \oslash \hat{\mathbf{c}}_{\text{exp}} \quad (\text{S29})$$

together with the relative statistical and systematic contributions:

$$\hat{\sigma}_{\text{exp,stat}}^{\circ 2} \oslash \hat{\sigma}_{\text{exp}}^{\circ 2} \odot \mathbf{CV}_{\text{exp}} = \hat{\sigma}_{\text{exp,stat}}^{\circ 2} \oslash (\hat{\sigma}_{\text{exp}} \odot \hat{\mathbf{c}}_{\text{exp}}) \quad (\text{S30a})$$

$$\hat{\sigma}_{\text{exp,sys}}^{\circ 2} \oslash \hat{\sigma}_{\text{exp}}^{\circ 2} \odot \mathbf{CV}_{\text{exp}} = \hat{\sigma}_{\text{exp,sys}}^{\circ 2} \oslash (\hat{\sigma}_{\text{exp}} \odot \hat{\mathbf{c}}_{\text{exp}}) \quad (\text{S30b})$$

are provided as well.

#### S1.4.1.4 Constant Activity Bias

As already noted in Sec. S1.1, for the radiation measurements conducted in this work, we assume that the activity of the radionuclides remains constant during the measurement time  $\Delta t^*$ . However, in reality, the activity of the radionuclide source changes with time [4]. Consequently, this assumption of a constant activity introduces a systematic bias in the spectral signature computation in Eq. S4. We can quantify this bias by comparing the mean number of decays  $N_{\text{const}}$  occurring during the measurement time  $\Delta t^*$  for a hypothetical radionuclide source with constant activity  $\mathcal{A}$ :

$$N_{\text{const}} = \mathcal{A} \Delta t^* \quad (\text{S31})$$

where:

|               |                  |    |
|---------------|------------------|----|
| $\mathcal{A}$ | source activity  | Bq |
| $\Delta t^*$  | measurement time | s  |

with the mean number of decays  $N_t$  occurring during the measurement time  $\Delta t^*$  for a real radionuclide source that decays according to the exponential decay law described by Eq. S26 into a stable nuclide:

$$N_t = \int_0^{\Delta t^*} \mathcal{A} \exp \left[ -\frac{\log(2)t}{t_{1/2}} \right] dt \quad (\text{S32a})$$

$$= \frac{\mathcal{A} t_{1/2}}{\log(2)} \left( 1 - \exp \left[ -\frac{\log(2) \Delta t^*}{t_{1/2}} \right] \right) \quad (\text{S32b})$$

where:

|               |                                                             |    |
|---------------|-------------------------------------------------------------|----|
| $\mathcal{A}$ | source activity at the start of the measurement ( $t = 0$ ) | Bq |
| $t_{1/2}$     | half-life                                                   | s  |
| $\Delta t^*$  | measurement time                                            | s  |

Combining Eqs. S31 and S32b, we may compute the relative error introduced by the constant activity assumption in the spectral signature as:

$$\frac{N_{\text{const}} - N_t}{N_t} = \frac{\log(2) \Delta t^*}{t_{1/2}} \left( 1 - \exp \left[ -\frac{\log(2) \Delta t^*}{t_{1/2}} \right] \right)^{-1} - 1 \quad (\text{S33})$$

From Eq. S33, two interesting observations can be made. First, the relative error is found to only depend on the half-life of the source and the measurement time  $\Delta t^*$ . In particular, it is found to be independent of the activity  $\mathcal{A}$  and consequently the measurement start time  $t$ . Second, for  $\Delta t^* \ll t_{1/2}$ , the relative error tends to  $\log(2) \Delta t^* / t_{1/2} - 1$ , which may provide a good approximation to estimate the relative error for long-lived radionuclides. For the radiation measurements conducted in the context of this work, relative errors introduced by the constant activity assumption are  $\ll 1\%$ .

## S1.4.2 Simulation Uncertainty

In this subsection, we focus on uncertainty estimates for the primary quantity of interest derived by the NPScinMC pipelines, that is the simulated spectral signature  $\hat{\mathbf{c}}_{\text{sim}} \in \mathbb{R}_+^{N_{\text{ch}} \times 1}$  (cf. Sec. S1.3). For a broader discussion on uncertainty estimation in Monte Carlo derived quantities, we refer to our earlier work [1].

### S1.4.2.1 Statistical Simulation Uncertainty

The main multivariate observable  $\mathbf{y} \in \mathbb{R}_+^{N_{\text{ch}} \times 1}$  derived from a simulated energy deposition event  $\tilde{n}_{\text{dep}}^*$  is equivalent to (cf. Sec. S1.3):

$$y_n = \begin{cases} \Phi\left(\frac{n + \frac{1}{2} - \tilde{n}_{\text{dep}}^*}{\sigma'_{\tilde{n}}(\tilde{n}_{\text{dep}}^*)}\right) - \Phi\left(\frac{n - \frac{1}{2} - \tilde{n}_{\text{dep}}^*}{\sigma'_{\tilde{n}}(\tilde{n}_{\text{dep}}^*)}\right) & \tilde{n}_{\text{dep}}^* > 0 \\ 0 & \tilde{n}_{\text{dep}}^* = 0 \end{cases} \quad (\text{S34a})$$

where:

|                            |                                                                          |
|----------------------------|--------------------------------------------------------------------------|
| $n$                        | pulse-height channel number                                              |
| $\tilde{n}_{\text{dep}}^*$ | continuous raw pulse-height channel number of an energy deposition event |
| $\sigma'_{\tilde{n}}$      | adapted spectral resolution standard deviation (cf. Eq. S14)             |

and with the pulse-height channel number being defined as  $\{n \in \mathbb{N}_+ \mid n \leq N_{\text{ch}}, N_{\text{ch}} = 1024\}$ . Note that we explicitly distinguish between the case of  $\tilde{n}_{\text{dep}}^* > 0$  and  $\tilde{n}_{\text{dep}}^* = 0$  in Eqs. S34a and S34b to emphasize that not all simulated primaries will result in an energy deposition event in one of the scintillation crystals. The number of recorded energy deposition events  $N_{\text{dep}}$  for a given acquisition channel is defined as  $N_{\text{dep}} = |\{\tilde{n}_{\text{dep}}^* \in \mathbb{R} \mid \tilde{n}_{\text{dep}}^* > 0\}|$ . Consequently, the number of simulated primaries not resulting in an energy deposition event in a given acquisition channel is given by  $N_0 = |\{\tilde{n}_{\text{dep}}^* \in \mathbb{R} \mid \tilde{n}_{\text{dep}}^* = 0\}|$ . Although we could record primary histories without energy depositions as zero-events in our Monte Carlo simulations, i.e.  $\{\mathbf{y}_i \in \mathbb{R}_+^{N_{\text{ch}} \times 1} \mid i \in \mathbb{N}_+, i \leq N_{\text{pr}}\}$ , this is not done in practice. Instead, we only record the energy deposition events  $\tilde{n}_{\text{dep}}^* > 0$  as  $\{\mathbf{y}_j \in \mathbb{R}_+^{N_{\text{ch}} \times 1} \mid j \in \mathbb{N}_+, j \leq N_{\text{dep}}\}$  and retrieve the number of zero-events by  $N_0 = N_{\text{pr}} - N_{\text{dep}}$ . The observable mean  $\bar{\mathbf{y}} \in \mathbb{R}_+^{N_{\text{ch}} \times 1}$  is then estimated by the arithmetic mean of the Monte Carlo sampled values  $\mathbf{y}_i$  as:

$$\bar{\mathbf{y}} = \frac{1}{N_{\text{pr}}} \sum_{i=1}^{N_{\text{pr}}} \mathbf{y}_i \quad (\text{S35a})$$

$$= \frac{1}{N_{\text{pr}}} \sum_{j=1}^{N_{\text{dep}}} \mathbf{y}_j \quad (\text{S35b})$$

$$\approx \frac{1}{N_{\text{pr}}} \mathbf{G} \mathbf{C}^+ \quad (\text{S35c})$$

where:

|                |                        |
|----------------|------------------------|
| $\mathbf{C}^+$ | prebinned count vector |
| $\mathbf{G}$   | Gaussian weight matrix |



In the last observable mean estimate Eq. S35c, we have utilized the Gaussian weight matrix  $\mathbf{G} \in \mathbb{R}_+^{N_{\text{ch}} \times N_{\text{ch}}^\dagger}$  and the prebinned count vector  $\mathbf{C}^\dagger \in \mathbb{N}^{N_{\text{ch}}^\dagger \times 1}$  introduced in Sec. S1.3. In the same way, we can estimate the standard deviation of the observable mean  $\sigma_{\bar{y}} \in \mathbb{R}_+^{N_{\text{ch}} \times 1}$  using the sample standard deviation [1, 42]:

$$\sigma_{\bar{y}} = \left\{ \frac{\sum_{i=1}^{N_{\text{pr}}} (\mathbf{y}_i - \bar{\mathbf{y}})^{\circ 2}}{N_{\text{pr}} (N_{\text{pr}} - 1)} \right\}^{\circ \frac{1}{2}} \quad (\text{S36a})$$

$$= \left\{ \frac{(N_{\text{pr}} - N_{\text{dep}}) \bar{\mathbf{y}}^{\circ 2} + \sum_{j=1}^{N_{\text{dep}}} (\mathbf{y}_j - \bar{\mathbf{y}})^{\circ 2}}{N_{\text{pr}} (N_{\text{pr}} - 1)} \right\}^{\circ \frac{1}{2}} \quad (\text{S36b})$$

$$\approx \left\{ \frac{(N_{\text{pr}} - N_{\text{dep}}) (\mathbf{G} \mathbf{C}^\dagger)^{\circ 2} + (N_{\text{pr}} \mathbf{G} - \mathbf{G} \mathbf{C}^\dagger \mathbf{J}_{1, N_{\text{ch}}^\dagger})^{\circ 2} \mathbf{C}^\dagger}{N_{\text{pr}}^3 (N_{\text{pr}} - 1)} \right\}^{\circ \frac{1}{2}} \quad (\text{S36c})$$

where we used again the matrix quantities introduced in Sec. S1.3 to approximate Eq. S36b with Eq. S36c. With  $\circ$ , we denote the Hadamard or element-wise power and  $\mathbf{J}_{m,n}$  is defined as a matrix of ones with dimension  $m \times n$ . Eqs. S36a–S36c quantify the statistical dispersion of the observable mean  $\bar{\mathbf{y}}$ . Consequently, we may estimate the statistical uncertainty of the simulated spectral signature  $\hat{\mathbf{c}}_{\text{sim}}$  by scaling the standard deviation of the observable mean  $\sigma_{\bar{y}}$  given by Eqs. S36a–S36c with the source geometry-matter factor  $F_{\text{src}}$  introduced in Sec. S1.3:

$$\hat{\sigma}_{\text{sim,stat}} = F_{\text{src}} \sigma_{\bar{y}} \quad (\text{S37})$$

As discussed in the main study, we select the number of primaries  $N_{\text{pr}}$  in such a way that  $\text{med}(\mathbf{C} \mathbf{V}_{\text{stat}}) = \text{med}(\hat{\sigma}_{\text{sim,stat}} \oslash \hat{\mathbf{c}}_{\text{sim}}) < 8\%$  over the spectral domain of interest in the acquisition channel #DET5 with  $\text{med}(\cdot)$  being the median operator and  $\mathbf{C} \mathbf{V}_{\text{stat}}$  the coefficient of variation vector with respect to the statistical simulation uncertainties.

The statistical uncertainty in Eq. S37 can in turn be quantified by the relative variance of the variance vector  $\mathbf{VOV}_{\bar{y}} \in \mathbb{R}_+^{N_{\text{ch}} \times 1}$  as [1, 43, 44]:

$$\mathbf{VOV}_{\bar{y}} \approx \frac{\sum_{i=1}^{N_{\text{pr}}} (\mathbf{y}_i - \bar{\mathbf{y}})^{\circ 4}}{\sum_{i=1}^{N_{\text{pr}}} (\mathbf{y}_i - \bar{\mathbf{y}})^{\circ 2}} - \frac{N_{\text{pr}} - 3}{N_{\text{pr}} - 1} \frac{1}{N_{\text{pr}}} \quad (\text{S38a})$$

$$= \frac{(N_{\text{pr}} - N_{\text{dep}}) \bar{\mathbf{y}}^{\circ 4} + \sum_{j=1}^{N_{\text{dep}}} (\mathbf{y}_j - \bar{\mathbf{y}})^{\circ 4}}{(N_{\text{pr}} - N_{\text{dep}}) \bar{\mathbf{y}}^{\circ 2} + \sum_{j=1}^{N_{\text{dep}}} (\mathbf{y}_j - \bar{\mathbf{y}})^{\circ 2}} - \frac{N_{\text{pr}} - 3}{N_{\text{pr}} - 1} \frac{1}{N_{\text{pr}}} \quad (\text{S38b})$$

$$\approx \frac{(N_{\text{pr}} - N_{\text{dep}}) (\mathbf{GC}^+) ^{\circ 4} + \left( N_{\text{pr}} \mathbf{G} - \mathbf{GC}^+ \mathbf{J}_{1, N_{\text{ch}}^+} \right) ^{\circ 4} \mathbf{C}^+}{N_{\text{pr}}^2 \left[ (N_{\text{pr}} - N_{\text{dep}}) (\mathbf{GC}^+) ^{\circ 2} + \left( N_{\text{pr}} \mathbf{G} - \mathbf{GC}^+ \mathbf{J}_{1, N_{\text{ch}}^+} \right) ^{\circ 2} \mathbf{C}^+ \right]} - \frac{N_{\text{pr}} - 3}{N_{\text{pr}} - 1} \frac{1}{N_{\text{pr}}} \quad (\text{S38c})$$

Given the definition of the relative variance of the variance (VOV) [1, 43, 44],  $\text{VOV}_{\bar{y}}$  is the same for the simulated spectral signature  $\hat{\mathbf{c}}_{\text{sim}}$ , i.e.  $\text{VOV}_{\bar{y}} = \text{VOV}_{\hat{\mathbf{c}}_{\text{sim}}}$ . As discussed in the main study, we select the number of primaries  $N_{\text{pr}}$  in such a way that  $\text{med}(\text{VOV}_{\hat{\mathbf{c}}_{\text{sim}}}) < 0.1\%$  over the spectral domain of interest in the acquisition channel #DET5.

### S1.4.2.2 Systematic Simulation Uncertainty

Similar to the measurement quantities discussed above, the simulated quantities are also subject to systematic uncertainties. In this work, we limit the systematic uncertainty analysis to the spectral meta-models applied in the postprocessing pipeline NPScinMC using the Monte Carlo sampling technique [45–47]. These models are the spectral energy and spectral resolution models with the related model parameters, i.e. the spectral energy bin width  $\Delta E'$ , the scale coefficient  $a_1$ , the power coefficient  $a_2$ , and the spectral intrinsic resolution standard deviation  $\sigma_{\tilde{n}, \text{intr}}$  (see Sec. S1.3). In line with the uncertainty quantification methodology [47], we interpret these model parameters as a random vector  $\mathbf{X} = (\Delta E', A_1^*, A_2, \sigma_{\tilde{n}, \text{intr}})^\top \in \mathbb{R}^{4 \times 1}$  with the log-transformed variable  $A_1^* := \log A_1$  and related marginal distribution:

$$\mathbf{X} \sim \mathcal{N}(\mathbf{x} \mid \boldsymbol{\mu}, \text{diag}(\sigma^{\circ 2}), \mathbf{x}_l, \mathbf{x}_u) \quad (\text{S39})$$

being the truncated multivariate normal distribution with mean  $\boldsymbol{\mu}$  and standard deviation  $\sigma$  defined by the regression results of the RLLCa1 pipeline. The truncation  $\mathbf{x}_l < \mathbf{x} < \mathbf{x}_u$  is set by  $\mathbf{x}_l = (-\infty, -\infty, 0, 0)^\top$  and  $\mathbf{x}_u = (\infty, \infty, \infty, \infty)^\top$ . To account for the statistical dependence between the scale coefficient  $a_1$  and the power coefficient  $a_2$ , we apply the copula theory to perform correlated sampling of these two parameters using the Gaussian copula  $\mathcal{C}_{\mathcal{N}}$  [48–50]:

$$\{A_1^*, A_2\} \sim \mathcal{C}_{\mathcal{N}} \left( F_{A_1^*}(a_1^*), F_{A_2}(a_2); \mathcal{R} \right) \quad (\text{S40a})$$

$$= \Phi_2 \left( \Phi^{-1} \left( F_{A_1^*}(a_1^*) \right), \Phi^{-1} \left( F_{A_2}(a_2) \right); \mathcal{R} \right) \quad (\text{S40b})$$

with the marginal cumulative distribution functions  $F$ , the inverse cumulative distribution function of the standard normal distribution  $\Phi^{-1}$  as well as the bivariate Gaussian cumulative distribution function  $\Phi_2$  with zero mean  $\mathbf{0}$  and correlation matrix  $\mathcal{R} \in \mathbb{R}^{3 \times 3}$  defined as:

$$\mathcal{R} = \begin{pmatrix} 1 & \text{corr}(a_1^*, a_2) \\ \text{corr}(a_2, a_1^*) & 1 \end{pmatrix} \quad (\text{S41})$$

The individual correlation coefficients  $\text{corr}(a_1^*, a_2) = \text{corr}(a_2, a_1^*)$  are provided by the regression analysis of the RLLCa1 pipeline (cf. Table S6). In contrast to the scale coefficient  $a_1$  and the power coefficient  $a_2$ , the spectral energy bin width  $\Delta E'$  and the spectral intrinsic resolution standard deviation  $\sigma_{\tilde{n}, \text{intr}}$  are sampled independently from the other parameters according to the corresponding marginal distribution given in Eq. S39. For more details on the copula theory, we recommend the monographs by Joe [49] and Nelsen [50].

Following a Monte Carlo approach, we draw a fixed number of  $N_{\text{sys}}$  independent samples  $\mathcal{X} = \{\mathbf{x}_i \in \mathbb{R}^{4 \times 1} \mid i \in \mathbb{N}_+, i \leq N_{\text{sys}}\}$  from the probabilistic input model detailed above. These samples are then propagated independently through the postprocessing pipeline NPScinMC discussed in Sec. S1.3. The resulting set of simulated spectral signatures  $\mathcal{Y} = \{\hat{\mathbf{c}}_{\text{sim},i} \in \mathbb{R}_+^{N_{\text{ch}} \times 1} \mid i \in \mathbb{N}_+, i \leq N_{\text{sys}}\}$  can then be used to estimate the systematic uncertainty by computing the sample standard deviation  $\hat{\sigma}_{\text{sim},\text{sys}} \in \mathbb{R}_+^{N_{\text{ch}} \times 1}$  as:

$$\hat{\sigma}_{\text{sim},\text{sys}} = \left[ \frac{N_{\text{sys}} \sum_{i=1}^{N_{\text{sys}}} \hat{\mathbf{c}}_{\text{sim},i}^{\circ 2} - \left( \sum_{i=1}^{N_{\text{sys}}} \hat{\mathbf{c}}_{\text{sim},i} \right)^{\circ 2}}{N_{\text{sys}}^2 (N_{\text{sys}} - 1)} \right]^{\circ \frac{1}{2}} \quad (\text{S42})$$

#### S1.4.2.3 Combined Simulation Uncertainty

In full analogy to the combined uncertainty estimation for the experimental spectral signature  $\hat{\mathbf{c}}_{\text{exp}}$  in Eq. S28a, the total or combined uncertainty  $\hat{\sigma}_{\text{sim}} \in \mathbb{R}_+^{N_{\text{ch}} \times 1}$  in the simulated spectral signature  $\hat{\mathbf{c}}_{\text{sim}}$  is estimated by combining the statistical and systematic uncertainties computed by Eqs. S37 and S42 in quadrature [32, 36]:

$$\hat{\sigma}_{\text{sim}} = \left( \hat{\sigma}_{\text{sim},\text{stat}}^{\circ 2} + \hat{\sigma}_{\text{sim},\text{sys}}^{\circ 2} \right)^{\circ \frac{1}{2}} \quad (\text{S43})$$

where:

|                                         |                                                             |                    |
|-----------------------------------------|-------------------------------------------------------------|--------------------|
| $\hat{\sigma}_{\text{sim},\text{stat}}$ | simulated statistical spectral signature standard deviation | $s^{-1}[\xi]^{-1}$ |
| $\hat{\sigma}_{\text{sim},\text{sys}}$  | simulated systematic spectral signature standard deviation  | $s^{-1}[\xi]^{-1}$ |

In this work,  $\hat{\sigma}_{\text{sim}}$  is indicated in each figure that presents simulated spectral signatures  $\hat{\mathbf{c}}_{\text{sim}}$ . If applicable, the coefficient of variation vector  $\mathbf{CV}_{\text{sim}} \in \mathbb{R}_+^{N_{\text{ch}} \times 1}$  defined as:

$$\mathbf{CV}_{\text{sim}} = \hat{\sigma}_{\text{sim}} \oslash \hat{\mathbf{c}}_{\text{sim}} \quad (\text{S44})$$

together with the relative statistical and systematic contributions:

$$\hat{\sigma}_{\text{sim},\text{stat}}^{\circ 2} \oslash \hat{\sigma}_{\text{sim}}^{\circ 2} \odot \mathbf{CV}_{\text{sim}} = \hat{\sigma}_{\text{sim},\text{stat}}^{\circ 2} \oslash (\hat{\sigma}_{\text{sim}} \odot \hat{\mathbf{c}}_{\text{sim}}) \quad (\text{S45a})$$

$$\hat{\sigma}_{\text{sim},\text{sys}}^{\circ 2} \oslash \hat{\sigma}_{\text{sim}}^{\circ 2} \odot \mathbf{CV}_{\text{sim}} = \hat{\sigma}_{\text{sim},\text{sys}}^{\circ 2} \oslash (\hat{\sigma}_{\text{sim}} \odot \hat{\mathbf{c}}_{\text{sim}}) \quad (\text{S45b})$$

are provided as well. In general, considering the spectral domain of interest  $\mathcal{D}_{\text{SDOI}}$  and the selected number of primaries (cf. Sec. S1.3), the systematic uncertainty is found to be dominant in distinct spectral features, particularly the FEPs, whereas the statistical uncertainty mainly affects the spectral continua of  $\hat{\mathbf{c}}_{\text{sim}}$  (see main study).

## S2 Supplementary Figures

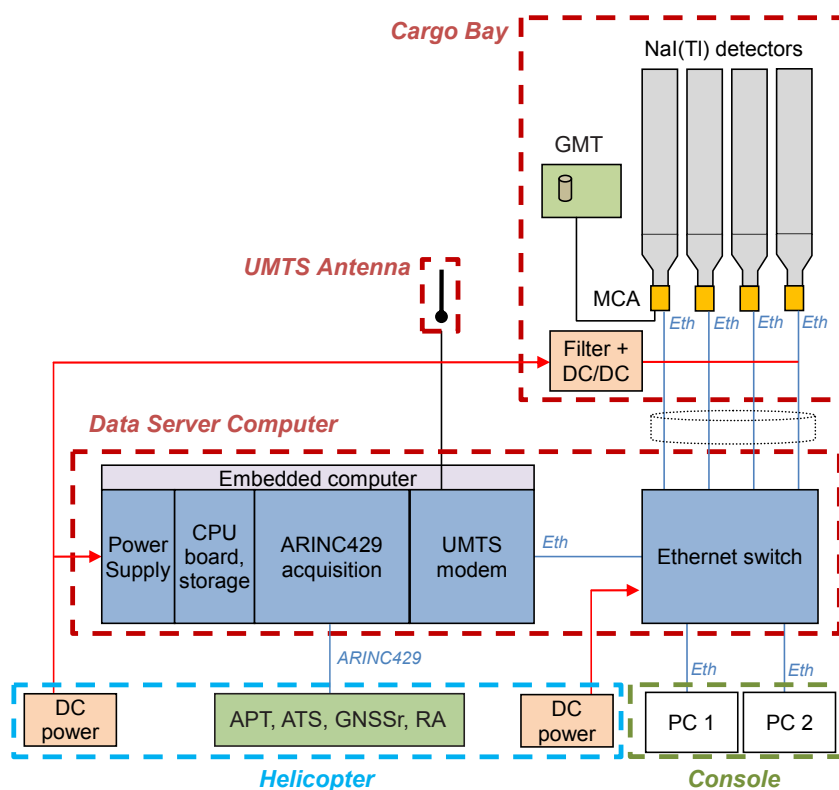

**Figure S4 System architecture of the Swiss AGRS system.** This scheme highlights the radiation detectors (NaI(Tl) scintillators and GMT: Geiger-Müller tube), detector electronics (MCA: multichannel analyzer), secondary helicopter sensors (APS: air pressure sensor, ATS: air temperature sensor, GNSSr: global navigation satellite system receiver, RA: radar altimeter), the rugged computer server, the operator consoles, the data transmission system (UMTS: universal mobile telecommunications system) as well as the data transmission standards (Eth: Ethernet, ARINC429: Mark 33 Digital Information Transfer System). Adapted from Perez et al. [51].

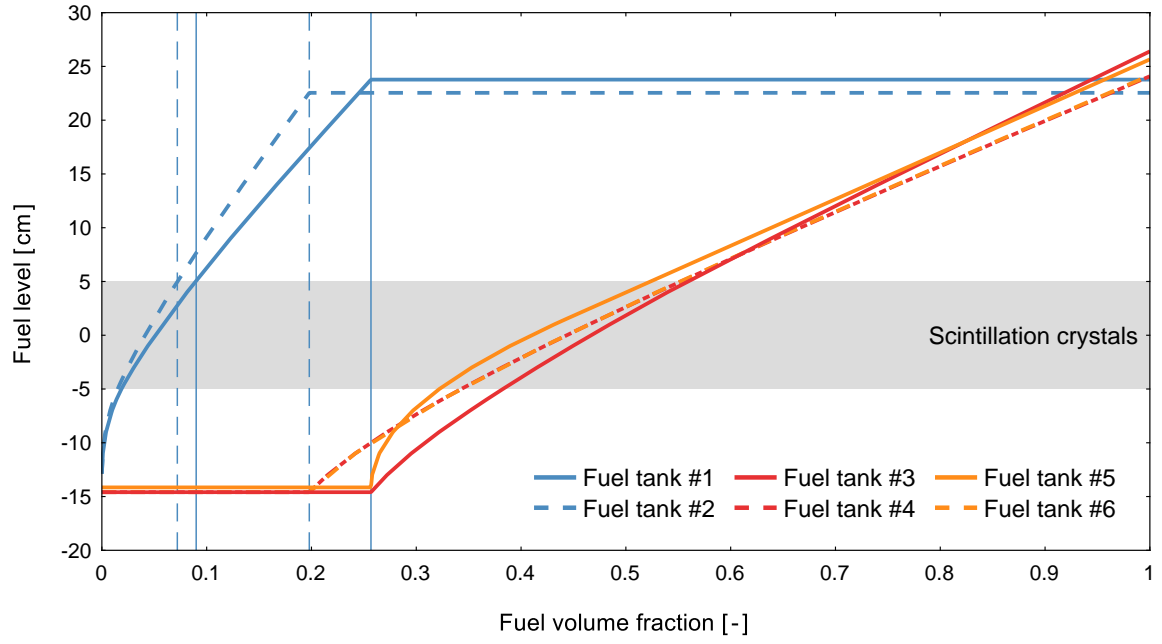

**Figure S5 Fuel level model of the AS332M1 aircraft.** In this graph, we present the fuel level model of the individual tanks #1 to #6 of the AS332M1 helicopter as a function of the fuel volume fraction  $\varrho_{\text{JF}}$  (total capacity  $1.988 \text{ m}^3$ ). The same numbering of the fuel tanks was used as in Fig. 2 in the main study. In addition, the diagram indicates the relative position of the scintillation crystals with respect to the fuel level in a horizontal flight configuration.

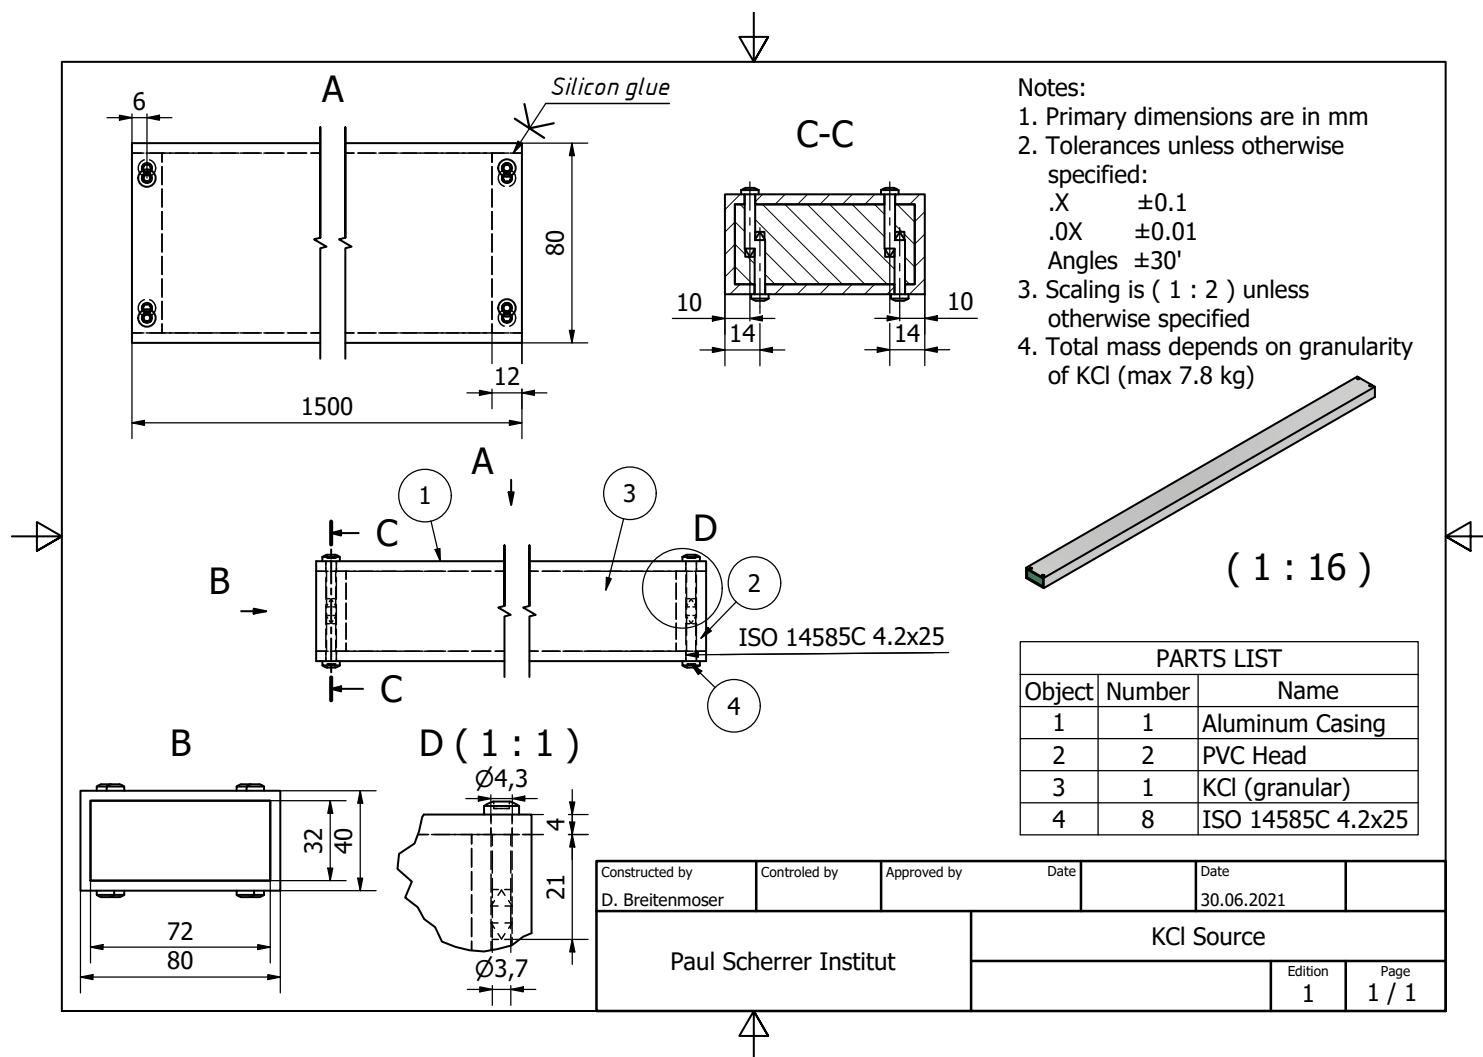

**Figure S6** Technical drawing of the custom-built  $K_{\text{nat}}$  sources. Here, we present a technical drawing of the custom-built  $K_{\text{nat}}$  sources that were deployed during the near-field radiation measurements at the Dübendorf Airfield.

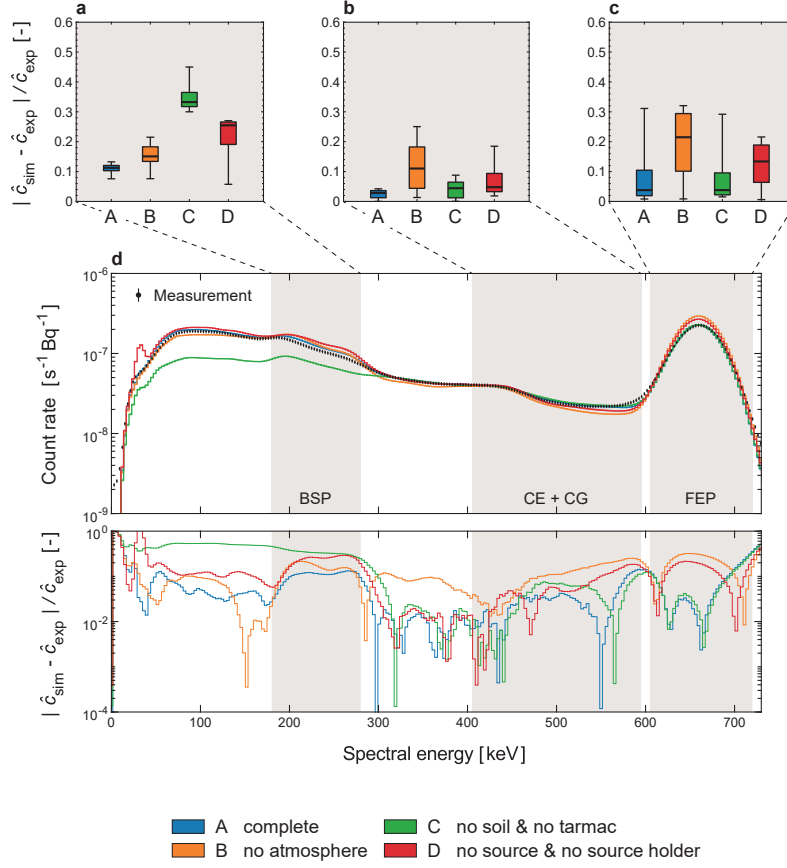

**Figure S7 Environment mass model sensitivity analysis.** Here, a mass model sensitivity analysis for the spectral signature of the  $^{137}_{55}\text{Cs}$  point source ( $\mathcal{A} = 9.0(5) \times 10^9 \text{ Bq}$ ) measured by the AGRS system (acquisition channel #DET5) in hover flight mode at a ground clearance of 31 m is presented. **a–c** Adjusted box plots [52, 53] characterizing the statistical distribution of the relative deviations  $|\hat{c}_{\text{sim}} - \hat{c}_{\text{exp}}| / \hat{c}_{\text{exp}}$  between the experimental ( $\hat{c}_{\text{exp}}$ ) and the simulated spectral signatures ( $\hat{c}_{\text{sim}}$ ) are shown for three different spectral domains (BSP: backscatter peak, CE+CG: Compton edge together with the Compton gap, FEP: full energy peak) and four different mass models A–D, in which the indicated media were removed and replaced with vacuum. The statistical analysis was performed using the Library for Robust Analysis (LIBRA) [54, 55]. **d** The measured ( $\hat{c}_{\text{exp}}$ ) and simulated ( $\hat{c}_{\text{sim}}$ ) mean spectral signatures for  $^{137}_{55}\text{Cs}$  are displayed as a function of the spectral energy  $E'$  with a spectral energy bin width of  $\Delta E' \sim 3 \text{ keV}$ . Spectral domains evaluated in a–c are highlighted. Uncertainties ( $\hat{\sigma}_{\text{exp}}$ ,  $\hat{\sigma}_{\text{sim}}$ ) are provided as 1 standard deviation shaded areas. In addition, the relative deviation  $|\hat{c}_{\text{sim}} - \hat{c}_{\text{exp}}| / \hat{c}_{\text{exp}}$  as a function of the spectral energy  $E'$  is displayed for all four mass models A–D. For further details on the provided spectral quantities, see Secs. S1.1–S1.4.

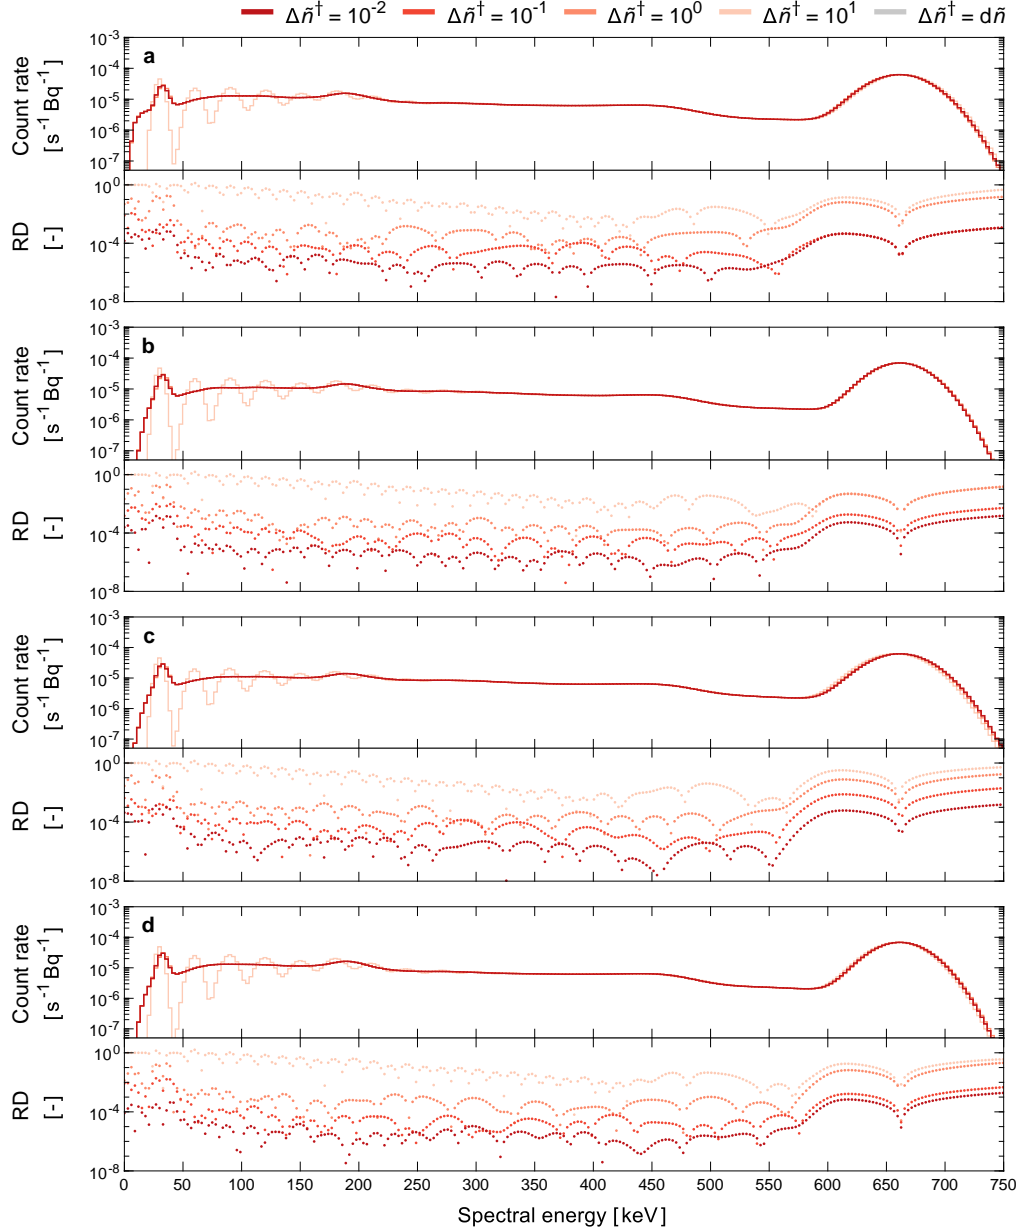

**Figure S8** These graphs present the results from a convergence study for the bin width  $\Delta\tilde{n}^\dagger$  of the refined pulse-height channel number  $\tilde{n}^\dagger$  introduced in the NPS<sub>cin</sub>MC pipeline (cf. Sec. S1.3). The simulated mean spectral signatures  $\hat{c}_{\text{sim}}$ , corresponding to four distinct bin widths  $\Delta\tilde{n}^\dagger = \{10^{-2}, 10^{-1}, 1, 10^1\}$  alongside the continuously convolved signature with  $\Delta\tilde{n}^\dagger = d\tilde{n}$  (hidden by the line width), are depicted as a function of the spectral energy  $E'$  with a spectral energy bin width of  $\Delta E' \sim 3$  keV for the four single acquisition channels #DET1–#DET4 (**a–d**). These simulations are based on the  $^{137}_{55}\text{Cs}$  calibration measurement described in Sec. S1.2 (see also [1]). In addition, the relative deviation (RD) between the continuously and discrete convolved signatures computed as  $|\hat{c}_{\text{sim},\Delta\tilde{n}^\dagger} - \hat{c}_{\text{sim},d\tilde{n}}|/\hat{c}_{\text{sim},d\tilde{n}}$  are provided. For further details on the provided spectral quantities, see Secs. S1.2 and S1.3.



## S3 Supplementary Tables

**Table S1**  $K_{\text{nat}}$  radionuclide source specification. Here, we present mass and activity data of the custom  $K_{\text{nat}}$  radionuclide sources deployed during the near-field radiation measurements at the Dübendorf Airfield.

| Source No.★ | KCl mass [kg]● | Activity [kBq]◦ |
|-------------|----------------|-----------------|
| 1           | 4.06(2)        | 66.6(10)        |
| 2           | 4.10(2)        | 67.3(10)        |
| 3           | 3.96(2)        | 65.0(10)        |
| 4           | 3.82(2)        | 62.7(9)         |
| 5           | 3.86(2)        | 63.3(10)        |
| 6           | 4.02(2)        | 66.0(10)        |
| 7           | 4.00(2)        | 65.6(10)        |
| sum         | 27.82(6)       | 456.6(26)       |

- ★ Custom source identifier.
- Mass of the granular KCl sealed in the corresponding sources, measured with a digital scale (model ICS435s-BC120/f/M).
- Activity  $A$  of  $^{40}\text{K}$ . The activity was determined following the methodology discussed by Breitenmoser [1], using nuclear data of  $^{40}\text{K}$  provided by Bé et al. [56] combined with molar mass data from Prohaska et al. [57] and isotopic abundance data from Meija et al. [58]. Uncertainties were computed by the standard error propagation methodology for independent variables [32, 37, 41] (cf. also to Sec. S1.4).

**Table S2** Near-field radiation measurements. Here, we present the gross and background measurement live time of the near-field radiation measurements performed at the Dübendorf Airfield.

| Measurement★ | Gross live time [min]● | Background live time [min]◦ |
|--------------|------------------------|-----------------------------|
| 0C           | 110                    | 28                          |
| 1E           | 180                    | 28                          |
| 1W           | 180                    | 48                          |
| 1N           | 180                    | 28                          |
| 1S           | 190                    | 48                          |
| 1NE          | 240                    | 65                          |
| 1SE          | 240                    | 65                          |
| 2E           | 780                    | 28                          |
| 2N           | 760                    | 48                          |
| 2S           | 780                    | 65                          |

- ★ Measurement identifier.
- Gross measurement live time  $t_{\text{gr}}$  for the corresponding measurement rounded to two significant digits.
- Background measurement live time  $t_{\text{b}}$  for the corresponding measurement rounded to two significant digits.

**Table S3 Mid-field radiation measurements.**  
Here, we present the gross and background measurement live time alongside the corresponding fuel volume fractions for the mid-field radiation measurements performed at the Thun military training ground.

| Fuel volume fraction★<br>[%] | Gross live time●<br>[s] | Background live time○<br>[s] |
|------------------------------|-------------------------|------------------------------|
| 9.5                          | 679                     | 897                          |
| 43.7                         | 995                     | 790                          |
| 92.2                         | 631                     | 814                          |

- ★ Fuel volume fraction  $\varrho_{\text{TF}}$  of the AS332M1 helicopter (total capacity: 1.988 m<sup>3</sup>) rounded to one decimal.
- Gross measurement live time  $t_{\text{gr}}$  rounded to three significant digits.
- Background measurement live time  $t_{\text{b}}$  rounded to three significant digits.

**Table S4 Far-field radiation measurements.**  
Here, we present the gross and background measurement live time alongside orientation and ground clearance data for the far-field radiation measurements performed at the Thun military training ground. Provided uncertainties represent the statistical standard deviation for the measurement (coverage factor  $k = 1$ ).

| Source★                         | $h_{\text{air}}^{\bullet}$<br>[m] | $-\alpha'^{\circ}$<br>[°] | $\beta'^{\dagger}$<br>[°] | $\gamma'^{\ddagger}$<br>[°] | $t_{\text{gr}}^{\S}$<br>[s] | $t_{\text{b}}^{\$}$<br>[s] |
|---------------------------------|-----------------------------------|---------------------------|---------------------------|-----------------------------|-----------------------------|----------------------------|
| <sup>133</sup> <sub>56</sub> Ba | 30.7(1)                           | 321(3)                    | 0.3(1)                    | −2.3(1)                     | 290                         | 314                        |
| <sup>133</sup> <sub>56</sub> Ba | 61.7(1)                           | 314(3)                    | 0.6(1)                    | −2.1(1)                     | 296                         | 285                        |
| <sup>133</sup> <sub>56</sub> Ba | 90.8(2)                           | 314(3)                    | 0.3(1)                    | −1.5(1)                     | 296                         | 260                        |
| <sup>137</sup> <sub>55</sub> Cs | 30.9(1)                           | 144(3)                    | −0.6(1)                   | −1.7(1)                     | 242                         | 263                        |
| <sup>137</sup> <sub>55</sub> Cs | 60.2(1)                           | 143(3)                    | −0.8(1)                   | −2.0(1)                     | 292                         | 307                        |
| <sup>137</sup> <sub>55</sub> Cs | 91.6(2)                           | 142(3)                    | −0.6(1)                   | −2.9(1)                     | 232                         | 298                        |

- ★ Radionuclide source adopted in the corresponding gross measurement.
- Mean ground clearance of the gross measurement determined by the radar altimeter of the AS332M1 helicopter. Note that the data was corrected for the vertical displacement between the radar altimeter, located at the bottom of the tail, and the spectrometer, mounted in the cargo bay (cf. Fig. 1 in the main study).
- Mean negative yaw angle relative to geographic north (cf. Fig. 2 in the main study).
- † Mean roll angle (cf. Fig. 2 in the main study).
- ‡ Mean pitch angle (cf. Fig. 2 in the main study).
- § Gross measurement live time  $t_{\text{gr}}$  rounded to three significant digits.
- \$ Background measurement live time  $t_{\text{b}}$  rounded to three significant digits.

**Table S5 Calibration sources.** This table lists the radionuclide sources and their associated photon emission lines used for laboratory calibration with the RLLCa1 pipeline.

| Nuclide                | Photon energy [keV] | References |
|------------------------|---------------------|------------|
| $^{40}_{19}\text{K}$   | 1460.822(6)         | [56]       |
| $^{60}_{27}\text{Co}$  | 1173.228(3)         | [59]       |
|                        | 1332.492(4)         | [59]       |
| $^{137}_{55}\text{Cs}$ | 661.657(3)          | [59]       |
| $^{152}_{63}\text{Eu}$ | 121.7817(3)         | [60]       |
|                        | 344.2785(12)        | [60]       |
| $^{208}_{81}\text{Tl}$ | 2614.511(10)        | [61]       |
| $^{214}_{82}\text{Pb}$ | 351.932(2)          | [62]       |
| $^{214}_{83}\text{Bi}$ | 609.312(7)          | [62]       |

**Table S6 Calibration results.** In this table, we present the calibration results derived by the RLLCa1 pipeline.

| Acquisition channel | $\Delta E' \star$<br>[keV] | $a_1^\bullet$<br>[-]    | $a_2^\circ$<br>[-]        | $\text{corr}(\log a_1, a_2)^\dagger$<br>[-] | $\mu_{\text{LLD}}^\ddagger$<br>[-] | $\sigma_{\text{LLD}}^\S$<br>[-] |
|---------------------|----------------------------|-------------------------|---------------------------|---------------------------------------------|------------------------------------|---------------------------------|
| #DET1               | 3.011(4)                   | $7.2(6) \times 10^{-1}$ | $6.01(16) \times 10^{-1}$ | $-9.89 \times 10^{-1}$                      | 5.37                               | 1.22                            |
| #DET2               | 3.0133(32)                 | $6.0(6) \times 10^{-1}$ | $6.29(17) \times 10^{-1}$ | $-9.91 \times 10^{-1}$                      | 5.59                               | 1.10                            |
| #DET3               | 3.0168(29)                 | $5.4(4) \times 10^{-1}$ | $6.68(14) \times 10^{-1}$ | $-9.90 \times 10^{-1}$                      | 6.14                               | 1.33                            |
| #DET4               | 3.013(4)                   | $5.7(6) \times 10^{-1}$ | $6.37(17) \times 10^{-1}$ | $-9.85 \times 10^{-1}$                      | 5.68                               | 1.79                            |
| #DET5               | 3.0141(23)                 | $5.9(5) \times 10^{-1}$ | $6.40(16) \times 10^{-1}$ | $-9.87 \times 10^{-1}$                      | 5.66                               | 1.34                            |

★ Spectral energy bin width (cf. Eq. S5).

● Scale coefficient of the spectral resolution model (cf. Eq. S7).

○ Power coefficient of the spectral resolution model (cf. Eq. S7).

† Correlation between the log-transformed scale coefficient  $\log a_1$  and the power coefficient  $a_2$  (rounded to three significant digits).

‡ Mean lower-level discriminator (rounded to three significant digits, cf. Eq. S10).

§ Lower-level discriminator standard deviation (rounded to three significant digits, cf. Eq. S10).

## Supplementary References

- [1] D. Breitenmoser, Towards Monte Carlo Based Full Spectrum Modeling of Airborne Gamma-Ray Spectrometry Systems, Doctoral Thesis, ETH Zurich, 2024. doi:10.3929/ethz-b-000694094.
- [2] D. Breitenmoser, F. Cerutti, G. Butterweck, M. M. Kasprzak, S. Mayer, Emulator-based Bayesian inference on non-proportional scintillation models by compton-edge probing, *Nature Communications* 14 (2023) 7790. doi:10.1038/s41467-023-42574-y.
- [3] W. L. Dunn, D. S. McGregor, J. K. Shultis, Gamma-Ray Spectroscopy, in: I. Fleck, M. Titov, C. Grupen, I. Buvat (Eds.), *Handbook of Particle Detection and Imaging*, Springer International Publishing, Cham, 2021, pp. 515–582. doi:10.1007/978-3-319-93785-4\_17.
- [4] G. F. Knoll, *Radiation Detection and Measurement*, John Wiley & Sons, New York, USA, 2010.
- [5] G. R. Gilmore, *Practical Gamma-Ray Spectrometry: Second Edition*, John Wiley and Sons, Chichester, UK, 2008. doi:10.1002/9780470861981.
- [6] D. Breitenmoser, G. Butterweck, M. M. Kasprzak, E. G. Yukihiro, S. Mayer, Experimental and Simulated Spectral Gamma-Ray Response of a NaI(Tl) Scintillation Detector used in Airborne Gamma-Ray Spectrometry, *Advances in Geosciences* 57 (2022) 89–107. doi:10.5194/ADGE0-57-89-2022.
- [7] W. Westmeier, The fitting of solid state detector spectra, *Nuclear Inst. and Methods in Physics Research, A* 242 (1986) 437–442. doi:10.1016/0168-9002(86)90442-0.
- [8] W. Westmeier, Techniques and problems of low-level gamma-ray spectrometry, *International Journal of Radiation Applications and Instrumentation Part A* 43 (1992) 305–322. doi:10.1016/0883-2889(92)90102-K.
- [9] H. X. Shi, B. X. Chen, T. Z. Li, D. Yun, Precise Monte Carlo simulation of gamma-ray response functions for an NaI(Tl) detector, *Applied Radiation and Isotopes* 57 (2002) 517–524. doi:10.1016/S0969-8043(02)00140-9.
- [10] R. P. Gardner, A. Sood, A Monte Carlo simulation approach for generating NaI detector response functions (DRFs) that accounts for non-linearity and variable flat continua, *Nuclear Instruments and Methods in Physics Research, Section B: Beam Interactions with Materials and Atoms* 213 (2004) 87–99. doi:10.1016/S0168-583X(03)01539-8.
- [11] M. J. Berger, S. M. Seltzer, Response functions for sodium iodide scintillation detectors, *Nuclear Instruments and Methods* 104 (1972) 317–332. doi:10.1016/0029-554X(72)90543-5.
- [12] N. Nelson, Y. Azmy, R. P. Gardner, J. Mattingly, R. Smith, L. G. Worrall, S. Dewji, Validation and uncertainty quantification of detector response functions for a 1"×2" NaI collimated detector intended for inverse radioisotope source mapping applications, *Nuclear Instruments and Methods in Physics Research, Section B: Beam Interactions with Materials and Atoms* 410 (2017) 1–15. doi:10.1016/j.nimb.2017.07.015.

- [13] M. Salathe, B. J. Quiter, M. S. Bandstra, J. C. Curtis, R. Meyer, C. H. Chow, Determining urban material activities with a vehicle-based multi-sensor system, *Physical Review Research* 3 (2021) 023070. doi:10.1103/PHYSREVRSEARCH.3.023070/FIGURES/11/MEDIUM.
- [14] R. G. Regis, C. A. Shoemaker, A Stochastic Radial Basis Function Method for the Global Optimization of Expensive Functions, *INFORMS Journal on Computing* 19 (2007) 497–509. doi:10.1287/IJOC.1060.0182.
- [15] H. M. Gutmann, A Radial Basis Function Method for Global Optimization, *Journal of Global Optimization* 2001 19:3 19 (2001) 201–227. doi:10.1023/A:1011255519438.
- [16] Y. Avni, Energy spectra of X-ray clusters of galaxies., *The Astrophysical Journal* 210 (1976) 642–646. doi:10.1086/154870.
- [17] S. A. Payne, N. J. Cherepy, G. Hull, J. D. Valentine, W. W. Moses, W. S. Choong, Non-proportionality of scintillator detectors: Theory and experiment, *IEEE Transactions on Nuclear Science* 56 (2009) 2506–2512. doi:10.1109/TNS.2009.2023657.
- [18] S. A. Payne, W. W. Moses, S. Sheets, L. Ahle, N. J. Cherepy, B. Sturm, S. Dazeley, G. Bizarri, W. S. Choong, Nonproportionality of scintillator detectors: Theory and experiment. II, *IEEE Transactions on Nuclear Science* 58 (2011) 3392–3402. doi:10.1109/TNS.2011.2167687.
- [19] H. Akima, A New Method of Interpolation and Smooth Curve Fitting Based on Local Procedures, *Journal of the ACM* 17 (1970) 589–602. doi:10.1145/321607.321609.
- [20] E. R. Van der Graaf, J. Limburg, R. L. Koomans, M. Tijs, Monte Carlo based calibration of scintillation detectors for laboratory and in situ gamma ray measurements, *Journal of Environmental Radioactivity* 102 (2011) 270–282. doi:10.1016/j.jenvrad.2010.12.001.
- [21] M. Baldoncini, M. Albéri, C. Bottardi, E. Chiarelli, K. G. C. Raptis, V. Strati, F. Mantovani, Investigating the potentialities of Monte Carlo simulation for assessing soil water content via proximal gamma-ray spectroscopy, *Journal of Environmental Radioactivity* 192 (2018) 105–116. doi:10.1016/j.jenvrad.2018.06.001.
- [22] J. C. Curtis, R. J. Cooper, T. H. Joshi, B. Cosofret, T. Schmit, J. Wright, J. Rameau, D. Konno, D. Brown, F. Otsuka, E. Rappeport, M. Marshall, J. Speicher, Simulation and validation of the Mobile Urban Radiation Search (MURS) gamma-ray detector response, *Nuclear Instruments and Methods in Physics Research, Section A: Accelerators, Spectrometers, Detectors and Associated Equipment* 954 (2020) 161128. doi:10.1016/j.nima.2018.08.087.
- [23] M. Maučec, R. J. De Meijer, C. Rigollet, P. H. Hendriks, D. G. Jones, Detection of radioactive particles offshore by  $\gamma$ -ray spectrometry Part I: Monte Carlo assessment of detection depth limits, *Nuclear Instruments and Methods in Physics Research, Section A: Accelerators, Spectrometers, Detectors and Associated Equipment* 525 (2004) 593–609. doi:10.1016/j.nima.2004.01.074.
- [24] E. G. Androulakaki, M. Kokkoris, C. Tsabaris, G. Eleftheriou, D. L. Patiris, F. K. Pappa, R. Vlastou, In situ  $\gamma$ -ray spectrometry in the marine environment using full spectrum analysis for natural radionuclides, *Applied Radiation and Isotopes* 114 (2016) 76–86. doi:10.1016/j.apradiso.2016.05.008.

- [25] T. H. Prettyman, J. J. Hagerty, R. C. Elphic, W. C. Feldman, D. J. Lawrence, G. W. McKinney, D. T. Vaniman, Elemental composition of the lunar surface: Analysis of gamma ray spectroscopy data from Lunar Prospector, *Journal of Geophysical Research: Planets* 111 (2006). doi:10.1029/2005JE002656.
- [26] T. H. Prettyman, N. Yamashita, R. C. Reedy, H. Y. McSween, D. W. Mittlefehldt, J. S. Hendricks, M. J. Toplis, Concentrations of potassium and thorium within Vesta's regolith, *Icarus* 259 (2015) 39–52. doi:10.1016/j.icarus.2015.05.035.
- [27] P. N. Peplowski, The global elemental composition of 433 Eros: First results from the NEAR gamma-ray spectrometer orbital dataset, *Planetary and Space Science* 134 (2016) 36–51. doi:10.1016/j.pss.2016.10.006.
- [28] J. D. Allyson, D. C. Sanderson, Monte Carlo simulation of environmental airborne gamma-spectrometry, *Journal of Environmental Radioactivity* 38 (1998) 259–282. doi:10.1016/S0265-931X(97)00040-4.
- [29] J. A. Kulisek, R. S. Wittman, E. A. Miller, W. J. Kernan, J. D. McCall, R. J. McConn, J. E. Schweppe, C. E. Seifert, S. C. Stave, T. N. Stewart, A 3D simulation look-up library for real-time airborne gamma-ray spectroscopy, *Nuclear Instruments and Methods in Physics Research, Section A: Accelerators, Spectrometers, Detectors and Associated Equipment* 879 (2018) 84–91. doi:10.1016/j.nima.2017.10.030.
- [30] C. Y. Yi, S. H. Hah, Monte Carlo calculation of response functions to gamma-ray point sources for a spherical NaI(Tl) detector, *Applied Radiation and Isotopes* 70 (2012) 2133–2136. doi:10.1016/j.apradiso.2012.02.081.
- [31] C. E. Rasmussen, C. K. I. Williams, *Gaussian Processes for Machine Learning*, MIT Press, Cambridge, Massachusetts, 2006. doi:10.7551/MITPRESS/3206.001.0001.
- [32] Joint Committee for Guides in Metrology, *Evaluation of Measurement Data — Guide to the Expression of Uncertainty in Measurement*, Technical Report, Bureau International des Poids et Mesures, 2008. URL: <https://www.iso.org/standard/50461.html>.
- [33] B. M. Ayyub, G. J. Klir, *Uncertainty Modeling and Analysis in Engineering and the Sciences*, Chapman and Hall/CRC, New York, 2006. doi:10.1201/9781420011456.
- [34] J. B. Nagel, *Bayesian Techniques for Inverse Uncertainty Quantification*, Doctoral Thesis, ETH Zurich, 2017. doi:10.3929/ethz-a-010835772.
- [35] A. D. Kiureghian, O. Ditlevsen, Aleatory or epistemic? Does it matter?, *Structural Safety* 31 (2009) 105–112. doi:10.1016/j.strusafe.2008.06.020.
- [36] Particle Data Group, R. L. Workman, V. D. Burkert, V. Crede, E. Klempt, U. Thoma, L. Tiator, K. Agashe, G. Aielli, B. C. Allanach, C. AMSler, M. Antonelli, E. C. Aschenauer, D. M. Asner, H. Baer, S. Banerjee, R. M. Barnett, L. Baudis, C. W. Bauer, J. J. Beatty, V. I. Belousov, J. Beringer, A. Bettini, O. Biebel, K. M. Black, E. Blucher, R. Bonventre, V. V. Bryzgalov, O. Buchmuller, M. A. Bychkov, R. N. Cahn, M. Carena, A. Ceccucci, A. Cerri, R. S. Chivukula, G. Cowan, K. Cranmer, O. Cremonesi, G. D'Ambrosio, T. Damour, D. de Florian, A. de Gouvêa, T. DeGrand, P. de Jong, S. Demers, B. A. Dobrescu, M. D'Onofrio, M. Doser, H. K. Dreiner, P. Eerola, U. Egede, S. Eidelman, A. X. El-Khadra, J. Ellis, S. C. Eno, J. Erler, V. V. Ezhela, W. Fetscher, B. D. Fields, A. Freitas, H. Gallagher, Y. Gershtein,

T. Gherghetta, M. C. Gonzalez-Garcia, M. Goodman, C. Grab, A. V. Gritsan, C. Grojean, D. E. Groom, M. Grünewald, A. Gurtu, T. Gutsche, H. E. Haber, M. Hamel, C. Hanhart, S. Hashimoto, Y. Hayato, A. Hebecker, S. Heinemeyer, J. J. Hernández-Rey, K. Hikasa, J. Hisano, A. Höcker, J. Holder, L. Hsu, J. Huston, T. Hyodo, A. Ianni, M. Kado, M. Karliner, U. F. Katz, M. Kenzie, V. A. Khoze, S. R. Klein, F. Krauss, M. Kreps, P. Križan, B. Krusche, Y. Kwon, O. Lahav, J. Laiho, L. P. Lellouch, J. Lesgourgues, A. R. Liddle, Z. Ligeti, C.-J. Lin, C. Lippmann, T. M. Liss, L. Littenberg, C. Lourenço, K. S. Lugovsky, S. B. Lugovsky, A. Lusiani, Y. Makida, F. Maltoni, T. Mannel, A. V. Manohar, W. J. Marciano, A. Masoni, J. Matthews, U.-G. Meißner, I.-A. Melzer-Pellmann, M. Mikhasenko, D. J. Miller, D. Milstead, R. E. Mitchell, K. Mönig, P. Molaro, F. Moortgat, M. Moskovic, K. Nakamura, M. Narain, P. Nason, S. Navas, A. Nelles, M. Neubert, P. Nevski, Y. Nir, K. A. Olive, C. Patrignani, J. A. Peacock, V. A. Petrov, E. Pianori, A. Pich, A. Piepke, F. Pietropaolo, A. Pomarol, S. Pordes, S. Profumo, A. Quadt, K. Rabbertz, J. Rademacker, G. Raffelt, M. Ramsey-Musolf, B. N. Ratcliff, P. Richardson, A. Ringwald, D. J. Robinson, S. Roesler, S. Rolli, A. Romaniouk, L. J. Rosenberg, J. L. Rosner, G. Rybka, M. G. Ryskin, R. A. Ryutin, Y. Sakai, S. Sarkar, F. Sauli, O. Schneider, S. Schönert, K. Scholberg, A. J. Schwartz, J. Schwiening, D. Scott, F. Sefkow, U. Seljak, V. Sharma, S. R. Sharpe, V. Shiltsev, G. Signorelli, M. Silari, F. Simon, T. Sjöstrand, P. Skands, T. Skwarnicki, G. F. Smoot, A. Soffer, M. S. Sozzi, S. Spanier, C. Spiering, A. Stahl, S. L. Stone, Y. Sumino, M. J. Syphers, F. Takahashi, M. Tanabashi, J. Tanaka, M. Taševský, K. Terao, K. Terashi, J. Terning, R. S. Thorne, M. Titov, N. P. Tkachenko, D. R. Tovey, K. Trabelsi, P. Urquijo, G. Valencia, R. Van de Water, N. Varelas, G. Venanzoni, L. Verde, I. Vivarelli, P. Vogel, W. Vogelsang, V. Vorobyev, S. P. Wakely, W. Walkowiak, C. W. Walter, D. Wands, D. H. Weinberg, E. J. Weinberg, N. Wermes, M. White, L. R. Wiencke, S. Willocq, C. G. Wohl, C. L. Woody, W.-M. Yao, M. Yokoyama, R. Yoshida, G. Zanderighi, G. P. Zeller, O. V. Zenin, R.-Y. Zhu, S.-L. Zhu, F. Zimmermann, P. A. Zyla, *Review of Particle Physics, Progress of Theoretical and Experimental Physics 2022* (2022) 083C01. doi:10.1093/ptep/ptac097.

- [37] P. R. Bevington, D. K. Robinson, *Data Reduction and Error Analysis for the Physical Sciences*, McGraw-Hill, 2003.
- [38] R. B. Abernethy, R. P. Benedict, R. B. Dowdell, ASME Measurement Uncertainty, *Journal of Fluids Engineering* 107 (1985) 161–164. doi:10.1115/1.3242450.
- [39] N. Tsoulfanidis, S. Landsberger, *Measurement and Detection of Radiation*, 4 ed., CRC Press, Boca Raton, 2015. doi:10.1201/b18203.
- [40] ISO 11929, *Determination of the Characteristic Limits (Decision Threshold, Detection Limit, and Limits of the Coverage Interval) for Measurements of Ionizing Radiation-Fundamental and Application*, Technical Report, International Organization for Standardization (ISO), Geneva, 2019.
- [41] H. H. Ku, Notes on the use of propagation of error formulas, *Journal of Research of the National Bureau of Standards* 70 (1966). URL: [http://nvlpubs.nist.gov/nistpubs/jres/70C/jresv70Cn4p263\\_A1b.pdf](http://nvlpubs.nist.gov/nistpubs/jres/70C/jresv70Cn4p263_A1b.pdf).
- [42] I. Lux, *Monte Carlo Particle Transport Methods*, CRC Press, Boca Raton, 2017. doi:10.1201/9781351074834.

- [43] R. A. Forster, T. E. Booth, S. P. Pederson, Ten new checks to assess the statistical quality of Monte Carlo solutions in MCNP, 8th international conference on radiation shielding (1994).
- [44] E. Cho, M. Jung Cho, J. Eltinge, The variance of sample variance from a finite population, *International Journal of Pure and Applied Mathematics* 21 (2005) 387–394.
- [45] D. Rochman, W. Zwermann, S. C. van der Marck, A. J. Koning, H. Sjöstrand, P. Helgesson, B. Krzykacz-Hausmann, Efficient Use of Monte Carlo: Uncertainty Propagation, *Nuclear Science and Engineering* 177 (2014) 337–349. doi:10.13182/NSE13-32.
- [46] P. Saracco, M. G. Pia, M. Batic, Theoretical Grounds for the Propagation of Uncertainties in Monte Carlo Particle Transport, *IEEE Transactions on Nuclear Science* 61 (2014) 877–887. doi:10.1109/TNS.2014.2300112.
- [47] B. Sudret, S. Marelli, J. Wiart, Surrogate models for uncertainty quantification: An overview, in: 2017 11th European Conference on Antennas and Propagation, EUCAP 2017, Institute of Electrical and Electronics Engineers Inc., 2017, pp. 793–797. doi:10.23919/EuCAP.2017.7928679.
- [48] A. Sklar, Fonctions de repartition an dimensions et leurs marges, *Publications de l’Institut Statistique de l’Université de Paris* 8 (1959) 229–231.
- [49] H. Joe, *Dependence Modeling with Copulas*, CRC Press, New York, USA, 2014. doi:10.1201/B17116/DEPENDENCE-MODELING-COPULAS-HARRY-JOE.
- [50] R. B. Nelsen, *An Introduction to Copulas*, Springer New York, Secaucus, NJ, USA, 2006. doi:10.1007/0-387-28678-0.
- [51] J. Perez, M. Guerin, L. Benelhadj, P. Monteil, Airworthy Radiometry System: Operating and Maintenance Manual, Technical Report DOC001938EN-G, Mirion Technologies Inc., 2018.
- [52] M. Hubert, E. Vandervieren, An adjusted boxplot for skewed distributions, *Computational Statistics & Data Analysis* 52 (2008) 5186–5201. doi:10.1016/j.csda.2007.11.008.
- [53] G. Brys, M. Hubert, A. Struyf, A Robust Measure of Skewness, *Journal of Computational and Graphical Statistics* 13 (2004) 996–1017. doi:10.1198/106186004X12632.
- [54] S. Verboven, M. Hubert, LIBRA: A MATLAB library for robust analysis, *Chemometrics and Intelligent Laboratory Systems* 75 (2005) 127–136. doi:10.1016/j.chemolab.2004.06.003.
- [55] S. Verboven, M. Hubert, MATLAB library LIBRA, *WIREs Computational Statistics* 2 (2010) 509–515. doi:10.1002/wics.96.
- [56] M.-M. Bé, V. Chisté, C. Dulieu, X. Mougeot, E. Browne, V. Chechev, N. Kuzmenko, F. Kondev, A. Luca, M. Galan, A. Nichols, A. Arinc, X. Huang, Table of Radionuclides (Vol. 5 - A = 22 to 244), Technical Report, Bureau International des Poids et Mesures, Sèvres, 2010. URL: <https://cea.hal.science/cea-02476352>.



- [57] T. Prohaska, J. Irrgeher, J. Benefield, J. K. Böhlke, L. A. Chesson, T. B. Coplen, T. Ding, P. J. H. Dunn, M. Gröning, N. E. Holden, H. A. J. Meijer, H. Moossen, A. Possolo, Y. Takahashi, J. Vogl, T. Walczyk, J. Wang, M. E. Wieser, S. Yoneda, X.-K. Zhu, J. Meija, Standard atomic weights of the elements 2021 (IUPAC Technical Report), *Pure and Applied Chemistry* 94 (2022) 573–600. doi:10.1515/pac-2019-0603.
- [58] J. Meija, T. B. Coplen, M. Berglund, W. A. Brand, P. D. Bièvre, M. Gröning, N. E. Holden, J. Irrgeher, R. D. Loss, T. Walczyk, T. Prohaska, Isotopic compositions of the elements 2013 (IUPAC Technical Report), *Pure and Applied Chemistry* 88 (2016) 293–306. doi:10.1515/pac-2015-0503.
- [59] M.-M. Bé, V. Chisté, C. Dulieu, E. Browne, C. Baglin, V. Chechev, N. Kuzmenko, R. L. Helmer, F. Kondev, T. Desmond Macmahon, Table of Radionuclides (Vol. 3 - A = 3 to 244), Technical Report, Bureau International des Poids et Mesures, Sèvres, 2006. URL: <https://cea.hal.science/cea-02476243>.
- [60] M.-M. Bé, V. Chisté, C. Dulieu, E. Browne, V. Chechev, N. Kuzmenko, R. L. Helmer, A. Nichols, E. Schönfeld, R. Dersch, Table of Radionuclides (Vol. 2 - A = 151 to 242), Technical Report, Bureau International des Poids et Mesures, Sèvres, 2004. URL: <https://cea.hal.science/cea-02476192>.
- [61] M.-M. Bé, V. Chisté, C. Dulieu, X. Mougeot, V. Chechev, F. Kondev, A. Nichols, X. Huang, B. Wang, Table of Radionuclides (Vol. 7 - A = 14 to 245), Technical Report, Bureau International des Poids et Mesures, Sèvres, 2013. URL: <https://cea.hal.science/cea-02476417>.
- [62] M.-M. Bé, V. Chisté, C. Dulieu, E. Browne, V. Chechev, N. Kuzmenko, F. Kondev, A. Luca, M. Galan, A. Pierce, X. Huang, Table of Radionuclides (Vol. 4 - A = 133 to 252), Technical Report, Bureau International des Poids et Mesures, Sèvres, 2008. URL: <https://cea.hal.science/cea-02476295>.
